# Supplementary material for: Variable screening based on Gaussian Centered L-moments
Source: arXiv:1908.11048 ancillary file (2019-08-29)
Supplement: Supplementary file 1 [file GCL_moments_arXiv_supplements.pdf]

# Supplementary material of "Variable Screening based on Gaussian Centered L-moments"

Hyowon An[a*], Kai Zhang[a], Hannu Oja[b] and J. S. Marron[a]

[a]*The University of North Carolina at Chapel Hill, Chapel Hill, North Carolina, USA;*
[b]*University of Turku, 20500 Turku, FI*

(*v1.0 released March 2018*)

## 1. Proofs of the theorems in the main paper

### 1.1. *Proof of Theorem 3.1*

*Lemma* 1.1 If $G^{-1} \circ F$ is convex on the support of $F$ and $\mu(F) = \mu(G)$, then there exist two points $0 < u_1 < u_2 < 1$ such that

$$G^{-1}(u) - F^{-1}(u) \geq 0 \text{ for } 0 < u \leq u_1 \text{ and } u_2 < u < 1,$$
$$G^{-1}(u) - F^{-1}(u) \leq 0 \text{ for } u_1 < u \leq u_2.$$

*Proof* Since the function $G^{-1} \circ F$ is convex, it meets the function $y = x$ at most twice. Suppose that the two functions meet less than twice. Then we have $G^{-1}(F(x)) - x > 0$ for all $x \in \mathbb{R}$ except at most one point $x'$ which implies $G^{-1}(u) > F^{-1}(u)$ for all $0 < u < 1$ except at most one point $u'$. However, this implies that

$$\mu(G) = \int_0^1 G^{-1}(u)\,\mathrm{d}u > \int_0^1 F^{-1}(u)\,\mathrm{d}u = \mu(F)$$

which contradicts the assumption $\mu(F) = \mu(G)$. Hence there exist two points $x_1, x_2 \in \mathbb{R}$ such that $G^{-1}(F(x)) - x \geq 0$ for all $x < x_1$ or $x > x_2$ and $G^{-1}(F(x)) - x \leq 0$ for all $x_1 \leq x \leq x_2$. This implies that there exist two points $u_1$ and $u_2$ such that $0 \leq u_1 < u_2 \leq 1$ and $G^{-1}(u) - F^{-1}(u) \geq 0$ for all $u \leq u_1$ or $u \geq u_2$ and $G^{-1}(u) - F^{-1}(u) \leq 0$ for all $u_1 \leq u \leq u_2$. ■

*Corresponding author. Email: ahwbest@gmail.com

*1.1.1. The first HL-moment satisfies Oja's criterion for a measure of location*

It can be seen from

$$\eta_1 = \int_0^1 F^{-1}(u) H_0\left(\Phi^{-1}(u)\right) \mathrm{d}u = \int_0^1 F^{-1}(u)\,\mathrm{d}u$$

that the first HL-moment is the mean. It was shown in Oja (1981) that the mean satisfies Oja's criteria for a measure of location.

*1.1.2. The second HL-moment satisfies Oja's criterion for a measure of scale*

To check whether $\eta_2$ satisfies the first condition of Oja's criteria (Definition 2.1.b), we let $G = F_{a,b}$ for $a > 0$. Then we have $G^{-1}(u) = aF^{-1}(u) + b$ for $0 < u < 1$. Now we have

$$\begin{aligned}
\eta_2(G) &= \int_0^1 G^{-1}(u)\Phi^{-1}(u)\,\mathrm{d}u \\
&= \int_0^1 \left\{aF^{-1}(u) + b\right\} \Phi^{-1}(u)\,\mathrm{d}u \\
&= a\int_0^1 F^{-1}(u)\Phi^{-1}(u)\,\mathrm{d}u + b\int_0^1 \Phi^{-1}(u)\,\mathrm{d}u \\
&= a\int_0^1 F^{-1}(u)\Phi^{-1}(u)\,\mathrm{d}u \\
&= a\eta_2(F).
\end{aligned} \tag{1}$$

Hence, we have $\eta(G) = a\eta(F)$ when $a > 0$. If we assume that $a < 0$, then we have $G^{-1}(u) = aF^{-1}(1-u) + b$. Following the same steps of derivation as Equation (1), we can obtain $\eta_2(G) = -a\eta_2(F)$. Combining these two results, we obtain $\eta_2(G) = |a|\eta_2(F)$.

To check the second condition of Definition 2.1.b, we see that

$$\begin{aligned}
G^{-1}(F(x)) - x \text{ is nondecreasing in } x &\Leftrightarrow \frac{f(x)}{g(G^{-1}(F(x)))} \geq 1 \\
&\Leftrightarrow \frac{1}{g(G^{-1}(u))} - \frac{1}{f(F^{-1}(u))} \geq 0 \\
&\Leftrightarrow G^{-1}(u) - F^{-1}(u) \text{ is nondecreasing in } u.
\end{aligned}$$

This yields $G^{-1}(u) - F^{-1}(u) - G^{-1}(1/2) + F^{-1}(1/2) \leq 0$ for $u \leq 1/2$ and $G^{-1}(u) - F^{-1}(u) - G^{-1}(1/2) + F^{-1}(1/2) \geq 0$ for $u \geq 1/2$. Now we have

$$\begin{aligned}
\eta_2(G) - \eta_2(F) &= \int_0^1 \left\{G^{-1}(u) - F^{-1}(u)\right\} \Phi^{-1}(u)\,\mathrm{d}u \\
&= \int_0^1 \left\{G^{-1}(u) - F^{-1}(u) - G^{-1}\left(\frac{1}{2}\right) + F^{-1}\left(\frac{1}{2}\right)\right\} \Phi^{-1}(u)\,\mathrm{d}u \\
&+ \int_0^1 \left\{G^{-1}\left(\frac{1}{2}\right) - F^{-1}\left(\frac{1}{2}\right)\right\} \Phi^{-1}(u)\,\mathrm{d}u \\
&\geq 0
\end{aligned}$$

where the last inequality results from the same signs of two functions inside the integral.

### *1.1.3. The HL-skewness satisfies Oja's criterion for a measure of skewness*

To check that $\eta_3^*$ satisfies the first condition of Definition 2.1.c, let $G = F_{a,b}$ for $a > 0$. Then we have

$$\begin{aligned}
\eta_3(G) &= \int_0^1 G^{-1}(u)\left\{\Phi^{-1}(u)^2 - 1\right\} \mathrm{d}u \\
&= \int_0^1 \left\{aF^{-1}(u) + b\right\}\left\{\Phi^{-1}(u)^2 - 1\right\} \mathrm{d}u \\
&= a\int_0^1 F^{-1}(u)\left\{\Phi^{-1}(u)^2 - 1\right\} \mathrm{d}u + b\int_0^1 \left\{\Phi^{-1}(u)^2 - 1\right\} \mathrm{d}u \\
&= a\int_0^1 F^{-1}(u)\left\{\Phi^{-1}(u)^2 - 1\right\} \mathrm{d}u \\
&= a\eta_3(F). \qquad (2)
\end{aligned}$$

Hence, we have $\eta_3(G) = a\eta_3(F)$ when $a > 0$. Following similar steps of derivation, it can be shown that $\eta_3(G) = a\eta_3(F)$ when $a < 0$. Combining these two results and $\eta_2(G) = |a|\eta_2(F)$, which comes from Subsubsection 1.1.2, we obtain the desired result $\eta_3^*(G) = \mathrm{sign}(a)\eta_3^*(F)$.

To check the second condition, we first assume that $\eta_1(F) = \eta_1(G) = 0$ and $\eta_2(F) = \eta_2(G) = 1$. Note that

$$\begin{aligned}
\eta_3(G) - \eta_3(F) &= \int_0^1 \left\{G^{-1}(u) - F^{-1}(u)\right\}\left\{\Phi^{-1}(u)^2 - 1\right\} \mathrm{d}u \\
&= \int_{-\infty}^{\infty} \left\{G^{-1}(\Phi(x)) - F^{-1}(\Phi(x))\right\}\phi(x)\left\{x^2 - 1\right\} \mathrm{d}x
\end{aligned}$$

By Lemma 1.1 and the monotonic increasing property of $\Phi(x)$, we know that there exist two points $x_1 < x_2$ such that $G^{-1}(\Phi(x)) - F^{-1}(\Phi(x)) \geq 0$ for $x \leq x_1$ or $x \geq x_2$ and $G^{-1}(\Phi(x)) - F^{-1}(\Phi(x)) \leq 0$ for $x_1 \leq x \leq x_2$. Now consider a polynomial $K(x|a, b) = H_2(x) + aH_1(x) + bH_0(x) = x^2 + ax + b - 1$ for $a \neq 0, b \in \mathbb{R}$. By equating $x^2 + ax + b - 1 = (x - x_1)(x - x_2)$ for all $x \in \mathbb{R}$, we can find two constants $a_{F,G}$ and $b_{F,G}$ such that $K(x|a_{F,G}, b_{F,G}) \geq 0$ for $x < x_1$ or $x > x_2$ and $K(x|a_{F,G}, b_{F,G}) \leq 0$ for $x_1 \leq x \leq x_2$.

Now we have

$$\begin{aligned}
0 &\leq \int_{-\infty}^{\infty} \phi(x)\left\{G^{-1}(\Phi(x)) - F^{-1}(\Phi(x))\right\} K(x|a_{F,G}, b_{F,G})\,\mathrm{d}x \\
&= \int_{-\infty}^{\infty} \phi(x)\left\{G^{-1}(\Phi(x)) - F^{-1}(\Phi(x))\right\}\{H_2(x) + a_{F,G}H_1(x) + b_{F,G}H_0(x)\}\,\mathrm{d}x \\
&= \{\eta_3(G) - \eta_3(F)\} + a_{F,G}\{\eta_2(G) - \eta_2(F)\} + b_{F,G}\{\eta_1(G) - \eta_1(F)\} \\
&= \eta_3(G) - \eta_3(F)
\end{aligned}$$

where the first inequality holds since the two functions $G^{-1}(\Phi(x)) - F^{-1}(\Phi(x))$ and

$K(x|a_{F,G}, b_{F,G})$ have the same sign for all $x \in \mathbb{R}$, and the last equality comes from the assumption that $\eta_1(F) = \eta_1(G) = 0$ and $\eta_2(F) = \eta_2(G) = 1$.

Now assume that two distributions $F$ and $G$ have arbitrary first and second HL-moment coefficients. Then we have

$$\eta_3^*(F) = \eta_3\left(F_{1/\eta_2(F), -\eta_1(F)/\eta_2(F)}\right) \leq \eta_3\left(G_{1/\eta_2(G), -\eta_1(G)/\eta_2(G)}\right) = \eta_3^*(G)$$

where the first and last equality holds since we showed that the first condition of Oja's criterion is satisfied.

### *1.1.4. The HL-kurtosis satisfies Oja's criterion for a measure of kurtosis*

To prove the theorem, we need the following lemmas.

*Lemma* 1.2 If $F$ is a symmetric distribution, then $\eta_3(F) = 0$.

*Proof* Since $F^{-1}$ is symmetric with respect to the point $(1/2, m(F))$, we have

$$F^{-1}(u) - m(F) = m(F) - F^{-1}(1-u) \tag{3}$$

for all $1/2 \leq u < 1$. We have

$$\begin{aligned} \eta_3(F) &= \int_0^{1/2} F^{-1}(u)\left\{\Phi^{-1}(u)^2 - 1\right\} \mathrm{d}u + \int_{1/2}^{1} F^{-1}(u)\left\{\Phi^{-1}(u)^2 - 1\right\} \mathrm{d}u \\ &= \int_0^{1/2} F^{-1}(u)\left\{\Phi^{-1}(u)^2 - 1\right\} \mathrm{d}u + \int_0^{1/2} F^{-1}(1-v)\left\{\Phi^{-1}(v)^2 - 1\right\} \mathrm{d}v \\ &= 2m(F)\int_0^{1/2} \Phi^{-1}(u)^2 - 1\,\mathrm{d}u \\ &= 0 \end{aligned}$$

where the second equation results from the change of variable $v = 1-u$ and the second to last equation results from Equation (3). ■

*Lemma* 1.3 Let $F$ and $G$ be symmetric distributions with the symmetry points $m(F)$ and $m(G)$ such that $\eta_1(F) = \eta_1(G) = 0$ and $\eta_2(F) = \eta_2(G) = 1$. If $G^{-1} \circ F$ is concave on $\{x|x < 0\}$ and convex on $\{x|x > 0\}$, then there exists two points $0 < u_1 < 1/2 < u_2 < 1$ such that

$$\begin{aligned} G^{-1}(u) - F^{-1}(u) \leq 0 \text{for} 0 < u \leq u_1 \text{ and } 1/2 < u \leq u_2, \\ G^{-1}(u) - F^{-1}(u) \geq 0 \text{for} u_1 < u \leq 1/2 \text{ and } u_2 < u \leq 1. \end{aligned}$$

*Proof* By the convexity assumption on $G^{-1} \circ F$, this function meets the function $y = x$ either once at $x = 0$ or three times at $x = x_1, 0, x_2$ such that $x_1 < x_2$ on the real line $\mathbb{R}$. Suppose that these two functions meet each other once. Then we have $G^{-1}(F(x)) - x < 0$

for $x < 0$ and $G^{-1}(F(x)) - x > 0$ for $x > 0$ which implies that

$$G^{-1}(u) - F^{-1}(u) < 0 \text{ for } u < \frac{1}{2} \text{ and } G^{-1}(u) - F^{-1}(u) > 0 \text{ for } u > \frac{1}{2} \tag{4}$$

since we assumed that $m(F) = 0$. We have

$$\begin{aligned}
\eta_2(G) &= \int_0^1 G^{-1}(u)\Phi^{-1}(u)\,\mathrm{d}u \\
&= \int_0^{1/2} G^{-1}(u)\Phi^{-1}(u)\,\mathrm{d}u + \int_{1/2}^1 G^{-1}(u)\Phi^{-1}(u)\,\mathrm{d}u \\
&> \int_0^{1/2} F^{-1}(u)\Phi^{-1}(u)\,\mathrm{d}u + \int_{1/2}^1 F^{-1}(u)\Phi^{-1}(u)\,\mathrm{d}u \\
&= \eta_2(F)
\end{aligned}$$

where the strict inequality holds owing to Equation (4). This contradicts the assumption $\eta_2(F) = \eta_2(G)$. Hence, $G^{-1}(F(x)) - x \leq 0$ for $x < x_1, 0 < x < x_2$ and $G^{-1}(F(x)) - x \geq 0$ for $x_1 < x < 0, x > x_2$. This indicates that there exist two points $u_1, u_2$ such that $0 < u_1 < 0 < u_2 < 1$ and $G^{-1}(u) - F^{-1}(u) \leq 0$ for $0 < u \leq u_1, 1/2 < u \leq u_2$ and $G^{-1}(u) - F^{-1}(u) \geq 0$ for $u_1 < u \leq 1/2, u_2 < u < 1$. ■

To check whether $\eta_4^*$ satisfies the first condition of Oja's criterion (Definition 2.1.d), we let $G = F_{a,b}$. First, assume that $a < 0$. Then we have

$$\begin{aligned}
\eta_4(G) &= \int_0^1 G^{-1}(u)\left\{\Phi^{-1}(u)^3 - 3\Phi^{-1}(u)\right\}\,\mathrm{d}u \\
&= \int_0^1 \left\{aF^{-1}(1-u) + b\right\}\left\{\Phi^{-1}(u)^3 - 3\Phi^{-1}(u)\right\}\,\mathrm{d}u \\
&= a\int_0^1 F^{-1}(1-u)\left\{\Phi^{-1}(u)^3 - 3\Phi^{-1}(u)\right\}\,\mathrm{d}u + b\int_0^1 \Phi^{-1}(u)^3 - 3\Phi^{-1}(u)\,\mathrm{d}u \\
&= -a\int_0^1 F^{-1}(u)\left\{\Phi^{-1}(u)^3 - 3\Phi^{-1}(u)\right\}\,\mathrm{d}u \\
&= -a\eta_4(F).
\end{aligned}$$

The case when $a > 0$ can be derived in a similar and easier way yielding $\eta_4(G) = a\eta_4(F)$. Combining these two results and $\eta_2(G) = |a|\eta_2(F)$, we obtain the desired result $\eta_4^*(G) = \eta_4^*(F)$.

To check the second condition, we first assume that $\eta_1(F) = \eta_1(G) = 0$ and $\eta_2(F) = \eta_2(G) = 1$. Since we have assumed that $F$ and $G$ are symmetric distributions, we have $\eta_3(F) = \eta_3(G) = 0$ by Lemma 1.2. Note that

$$\begin{aligned}
\eta_4(G) - \eta_4(F) &= \int_0^1 \left\{G^{-1}(u) - F^{-1}(u)\right\}\left\{\Phi^{-1}(u)^3 - 3\Phi^{-1}(u)\right\}\,\mathrm{d}u \\
&= \int_{-\infty}^{\infty} \left\{G^{-1}(\Phi(x)) - F^{-1}(\Phi(x))\right\}\phi(x)\left\{x^3 - 3x\right\}\,\mathrm{d}x
\end{aligned}$$

By Lemma 1.3 and the monotonic increasing property of $\Phi(x)$, we know that there exist two points $x_1 < 0 < x_2$ and $G^{-1}(\Phi(x)) - F^{-1}(\Phi(x)) \geq 0$ for $x_1 < x < 0$ and $x > x_2$, and $G^{-1}(\Phi(x)) - F^{-1}(\Phi(x)) \leq 0$ for $x < x_1$ and $0 \leq x \leq x_2$. Now consider a polynomial $K(x|a,b,c) = H_3(x) + aH_2(x) + bH_1(x) + cH_0(x) = x^3 - 3x + a(x^2-1) + bx + c = x^3 + ax^2 + (b-3)x + c - a$ for some $a, b$ and $c$. By equating

$$x^3 + ax^2 + (b-3)x + c - a = x(x-x_1)(x-x_2) \tag{5}$$

for all $x \in \mathbb{R}$, we can find $a_{F,G}, b_{F,G}$ and $c_{F,G}$ such that $K(x|a_{F,G}, b_{F,G}, c_{F,G}) \geq 0$ for $x_1 \leq x \leq 0$ and $x \geq x_2$, $K(x|a_{F,G}, b_{F,G}, c_{F,G}) \leq 0$ for $x \leq x_1$ and $0 \leq x \leq x_2$. Note that $a_{F,G} = c_{F,G}$ should hold from the equation (5). Now we have

$$\begin{aligned}
0 &\leq \int_{-\infty}^{\infty} \phi(x) \left\{G^{-1}(\Phi(x)) - F^{-1}(\Phi(x))\right\} K(x|a_{F,G}, b_{F,G}, c_{F,G})\,\mathrm{d}x \\
&= \int_{-\infty}^{\infty} \phi(x) \left\{G^{-1}(\Phi(x)) - F^{-1}(\Phi(x))\right\} \\
&\qquad \times \{H_3(x) + a_{F,G}H_2(x) + b_{F,G}H_1(x) + c_{F,G}H_0(x)\}\,\mathrm{d}x \\
&= \{\eta_4(G) - \eta_4(F)\} + a_{F,G}\{\eta_3(G) - \eta_3(F)\} + b_{F,G}\{\eta_2(G) - \eta_2(F)\} \\
&+ c_{F,G}\{\eta_1(G) - \eta_1(F)\} \\
&= \eta_4(G) - \eta_4(F).
\end{aligned}$$

Now assume that two distributions $F$ and $G$ have arbitrary first and second HL-moment values. Then we have

$$\eta_4^*(F) = \eta_4\left(F_{1/\eta_2(F), -\eta_1(F)/\eta_2(F)}\right) \leq \eta_4\left(G_{1/\eta_2(G), -\eta_1(G)/\eta_2(G)}\right) = \eta_4^*(G)$$

where the first and last equality holds since we showed that the first condition of Oja's criterion is satisfied.

## 1.2. *Proof of Theorem 3.2*

Note that

$$\begin{aligned}
&\frac{1}{r}\sum_{k=0}^{r-2}(-1)^k \binom{r-2}{k} E\left(X_{(r-k):r} - X_{(r-k-1):r}\right) \\
= \;&\frac{1}{r}\sum_{k=1}^{r-2}\left\{(-1)^k\binom{r-2}{k} - (-1)^{k-1}\binom{r-2}{k-1}\right\} EX_{(r-k):r} \\
&+\frac{1}{r}EX_{r:r} - \frac{1}{r}(-1)^{r-2}EX_{1:r}.
\end{aligned} \tag{6}$$

We have

$$(-1)^k\binom{r-2}{k} - (-1)^{k-1}\binom{r-2}{k-1} = (-1)^k\binom{r-1}{k}.$$

Substituting this equation into Equation (6) yields

$$\frac{1}{r}\sum_{k=0}^{r-2}(-1)^k \left(\begin{array}{c} r-2 \\ k \end{array}\right) E\left(X_{(r-k):r} - X_{(r-k-1):r}\right) = \frac{1}{r}\sum_{k=0}^{r-1}(-1)^k \left(\begin{array}{c} r-1 \\ k \end{array}\right) EX_{(r-k):r} = \lambda_r$$

where the last equality results from Equation (2.1) of Hosking (1990).

### 1.3. ***Proof of Theorem 3.3***

The first three equations in Theorem 3.3 of the main paper are obvious from Equation (13) of that paper. Note from Equation (3.3.1') of David and Nagaraja (2003) that

$$E\left(X_{j:r}\right) = \frac{r!}{(j-1)!(r-j)!}\int_0^1 F^{-1}(u)u^{j-1}(1-u)^{r-j}\,\mathrm{d}u.$$

From this equation, we have

$$\begin{aligned} E\left(X_{3:4} - X_{2:4}\right) &= 12\int_0^1 F^{-1}(u)\left\{u^2(1-u) - u(1-u)^2\right\}\mathrm{d}u \\ &= \int_0^1 F^{-1}(u)\left(-24u^3 + 36u^2 - 12u\right)\mathrm{d}u. \end{aligned} \tag{7}$$

In addition, note from Equation (2.2) of Hosking (1990) that we have

$$\begin{aligned} \lambda_2 &= \int_0^1 F^{-1}(u)\,(2u-1)\;\mathrm{d}u, \\ \lambda_4 &= \int_0^1 F^{-1}(u)\left(20u^3 - 30u^2 + 12u - 1\right)\mathrm{d}u. \end{aligned} \tag{8}$$

Combining Equations (7) and (8) yields the following equation,

$$-6\left(\lambda_4 - \lambda_2\right) = 5E\left(X_{3:4} - X_{2:4}\right).$$

Note from Equation (13) of the main paper that we have

$$\begin{aligned}
\rho_{F_0,4} &= \frac{1}{4}\left\{\frac{1}{\delta_{3,4:4}(F_0)}E(X_{4:4}-X_{3:4}) - \frac{2}{\delta_{2,3:4}(F_0)}E(X_{3:4}-X_{2:4})\right.\\
&\qquad \left. + \frac{1}{\delta_{1,2:4}(F_0)}E(X_{2:4}-X_{1:4})\right\}\\
&= \frac{1}{4\delta_{3,4:4}(F_0)}\left\{E(X_{4:4}-X_{3:4}) - 2\frac{\delta_{3,4:4}(F_0)}{\delta_{2,3:4}(F_0)}E(X_{3:4}-X_{2:4}) + E(X_{2:4}-X_{1:4})\right\}\\
&= \frac{1}{4\delta_{3,4:4}(F_0)}\left[4\lambda_4 - 2\left\{\frac{\delta_{3,4:4}(F_0)}{\delta_{2,3:4}(F_0)} - 1\right\}E(X_{3:4}-X_{2:4})\right]\\
&= \frac{\lambda_4}{\delta_{3,4:4}(F_0)} - \frac{1}{2}\left\{\frac{1}{\delta_{2,3:4}(F_0)} - \frac{1}{\delta_{3,4:4}(F_0)}\right\}\left\{-\frac{6}{5}(\lambda_4-\lambda_2)\right\}\\
&= \left\{\frac{3}{5}\frac{1}{\delta_{2,3:4}(F_0)} + \frac{2}{5}\frac{1}{\delta_{3,4:4}(F_0)}\right\}\lambda_4 - \frac{3}{5}\left\{\frac{1}{\delta_{2,3:4}(F_0)} - \frac{1}{\delta_{3,4:4}(F_0)}\right\}\lambda_2,
\end{aligned}$$

where the second equality results from $\delta_{1,2:4}(F_0) = \delta_{3,4:4}(F_0)$ because of the symmetry of $F_0$. Hence, the 4th rescaled L-moment ratio based on the distribution $F_0$, $\rho^*_{F_0,4}$, satisfies

$$\begin{aligned}
\rho^*_{F_0,4} &= \frac{\rho_{F_0,4}}{\rho_{F_0,2}}\\
&= \frac{\delta_{1,2:2}(F_0)}{5}\left\{\frac{3}{\delta_{2,3:4}(F_0)} + \frac{2}{\delta_{3,4:4}(F_0)}\right\}\lambda_4^* - \frac{3\delta_{1,2:2}(F_0)}{5}\left\{\frac{1}{\delta_{2,3:4}(F_0)} - \frac{1}{\delta_{3,4:4}(F_0)}\right\}.
\end{aligned}$$

We show that $\rho^*_{F_0,4}$ satisfies Oja's criteria for a measure of kurtosis given in Definition 2.2.d. The proofs for $\rho_{F_0,2}$ and $\rho^*_{F_0,3}$ follow similar steps with the proof for $\rho^*_{F_0,4}$. Let

$$\begin{aligned}
\alpha_{F_0} &= \frac{\delta_{1,2:2}(F_0)}{5}\left\{\frac{3}{\delta_{2,3:4}(F_0)} + \frac{2}{\delta_{3,4:4}(F_0)}\right\},\\
\beta_{F_0} &= -\frac{3\delta_{1,2:2}(F_0)}{5}\left\{\frac{1}{\delta_{2,3:4}(F_0)} - \frac{1}{\delta_{3,4:4}(F_0)}\right\},
\end{aligned}$$

so that we have $\rho^*_{F_0,4} = \alpha_{F_0}\lambda_4^* + \beta_{F_0}$. For any two real numbers $a \neq 0$ and $b \in \mathbb{R}$, we have

$$\begin{aligned}
\rho^*_{F_0,4}(F_{a,b}) &= \alpha_{F_0}\lambda_4^*(F_{a,b}) + \beta_{F_0}\\
&= \alpha_{F_0}\lambda_4^*(F) + \beta_{F_0}\\
&= \rho^*_{F_0,4}(F),
\end{aligned}$$

since $\lambda_4^*$ satisfies Oja's critera for a measure of kurtosis as shown in Hosking (1989). In addition, suppose that $F, G \in \mathcal{F}_s$, $G^{-1} \circ F$ is concave on $\{x|x \leq m(F)\}$ and convex on $\{x|x > m(F)\}$. Then we have

$$\rho^*_{F_0,4}(F) = \alpha_{F_0}\lambda^*_{F_0,4}(F) + \beta_{F_0} \leq \alpha_{F_0}\lambda^*_{F_0,4}(G) + \beta_{F_0} = \rho^*_{F_0,4}(G),$$

since $\alpha_{F_0} > 0$ and $\lambda_4^*$ satisfies Oja's criteria for a measure of kurtosis.

## 1.4. *Proof of Theorem 6.2*

The following lemmas are needed in this subsection.

*Lemma* 1.4 Let $\theta : \mathcal{F} \to \mathbb{R}$ be an L-functional in the form (5) of the main paper. If $\theta$ is a symmetric L-functional and $F$ is a symmetric distribution, then we have $\mathrm{SIF}(x; F, \theta) = \mathrm{IF}(x; F, \theta)$ for all $x \in \mathbb{R}$.

*Proof* From Equation (5.35) of Huber and Ronchetti (2009), if both the functional $\theta$ and distribution $F$ are symmetric, then we have

$$\mathrm{IF}(x; F, \theta) = \mathrm{IF}(-x; F, \theta). \tag{9}$$

Let $Q_u : \mathcal{F} \to \mathbb{R}$ be a functional such that $Q_u(F) = F^{-1}(u)$. Then it can be seen from Equations (3.46) and (3.47) of Huber and Ronchetti (2009) that

$$\mathrm{SIF}\left(x, F, Q_u\right) = \frac{1}{2}\left\{\mathrm{IF}\left(-x; F, Q_u\right) + \mathrm{IF}\left(x; F, Q_u\right)\right\}.$$

It can be seen using this result and the first equality in Equation (3.49) of Huber and Ronchetti (2009) that

$$\mathrm{SIF}(x, F, \theta) = \frac{1}{2}\{\mathrm{IF}(-x; F, \theta) + \mathrm{IF}(x; F, \theta)\}.$$

Combining this equation and Equation (9), we obtain the desired result. ■

*Lemma* 1.5 For a functional $\theta = \theta_1/\theta_2$ such that $\theta_1, \theta_2 : \mathcal{F} \to \mathbb{R}$, we have

$$\mathrm{IF}(x; F, \theta) = \frac{\theta_2(F)\mathrm{IF}(x; F, \theta_1) - \theta_1(F)\mathrm{IF}(x; F, \theta_2)}{\theta_2(F)^2},$$
$$\mathrm{SIF}(x; F, \theta) = \frac{\theta_2(F)\mathrm{SIF}(x; F, \theta_1) - \theta_1(F)\mathrm{SIF}(x; F, \theta_2)}{\theta_2(F)^2}$$

since both the influence and symmetric influence functions are right-hand derivatives of a function. ■

Since $\eta_4^*$ satisfies Oja's criteria for a measure of kurtosis and $\eta_2$ satisfies Oja's criteria for a measure of scale by Theorem 3.1 of the main paper, they satisfy $\eta_4^*(F) = \eta_4^*\left(F_{-1,0}\right)$ and $\eta_2(F) = \eta_2\left(F_{-1,0}\right)$ for all $F \in \mathcal{F}$. Hence, we have $\eta_4(F) = \eta_4\left(F_{-1,0}\right)$ for all $F \in \mathcal{F}$ so both the functionals $\eta_2$ and $\eta_4$ are symmetric L-functionals. By Lemma 1.4, we have $\mathrm{SIF}\left(x; F, \eta_2\right) = \mathrm{IF}\left(x; F, \eta_2\right)$ and $\mathrm{SIF}\left(x; F, \eta_4\right) = \mathrm{IF}\left(x; F, \eta_4\right)$ since $F$ is a symmetric

distribution. By Lemma 1.5, we have

$$\begin{aligned}\mathrm{SIF}\left(x;F,\eta_4^*\right) &= \frac{\eta_2(F)\mathrm{SIF}\left(x;F,\eta_4\right)-\eta_4(F)\mathrm{SIF}\left(x;F,\eta_2\right)}{\eta_2(F)^2}\\ &= \frac{\eta_2(F)\mathrm{IF}\left(x;F,\eta_4\right)-\eta_4(F)\mathrm{IF}\left(x;F,\eta_2\right)}{\eta_2(F)^2}\\ &= \mathrm{IF}\left(x;F,\eta_4^*\right).\end{aligned}$$

Following the same steps of derivation, it can be shown that $\mathrm{SIF}\left(x;F,\lambda_4^*\right)=\mathrm{IF}\left(x;F,\lambda_4^*\right)$ and $\mathrm{SIF}\left(x;F,\rho_4^*\right)=\mathrm{IF}\left(x;F,\rho_4^*\right)$.

## 1.5. ***Proof of Theorem 6.3***

Chapter 3 of Cormen et al. (2009) shows some definitions and theorems about asymptotic bounds. We use slightly different versions in this paper.

*Definition* 1.1 Let $J_1,J_2:\mathbb{R}\to\mathbb{R}$. We write

(1) $J_1(x)=\Theta\left(J_2(x)\right)$ if $\exists a_1,a_2,x'>0$ s.t. $a_1\left|J_2(x)\right|\le\left|J_1(x)\right|\le a_2\left|J_2(x)\right|\quad\forall|x|\ge x'$,
(2) $J_1(x)=O\left(J_2(x)\right)$ if $\exists a,x'>0$ s.t. $\left|J_1(x)\right|\le a\left|J_2(x)\right|\quad\forall|x|\ge x'$,
(3) $J_1(x)=\Omega\left(J_2(x)\right)$ if $\exists a,x'>0$ s.t. $a\left|J_2(x)\right|\le\left|J_1(x)\right|\quad\forall|x|\ge x'$,
(4) $J_1(x)=o\left(J_2(x)\right)$ if $\lim_{x\to\infty}\frac{|J_1(x)|}{|J_2(x)|}=\lim_{x\to-\infty}\frac{|J_1(x)|}{|J_2(x)|}=0$.

Note that the asymptotic bounds are defined in terms of both-sides limits. We write the right-side asymptotic bound as

$$J_1(x)=\Theta\left(J_2(x)\right)\ \text{ as } x\to\infty$$

if there exist $a_1,a_2,x'>0$ such that $a_1\left|J_2(x)\right|\le\left|J_1(x)\right|\le a_2\left|J_2(x)\right|$ for all $x\ge x'$. The left-side asymptotic bound is defined in the opposite way as $x\to-\infty$. We define the right- and left-side asymptotic bounds in the same way for the other notations; $O$, $\Omega$ and $o$. ■

It can be easily seen that we have $J_1(x)=\Theta\left(J_2(x)\right)$ if and only if $J_1(x)=\Theta\left(J_2(x)\right)$ as $x\to\infty$ and $x\to-\infty$. The same holds when $\Theta$ is replaced by $O,\Omega$ and $o$.

*Lemma* 1.6 Let $J_1,J_2:\mathbb{R}\to\mathbb{R}$ be two functions.

(1) If $J_1(x)=o\left(J_2(x)\right)$, then $J_1(x)+J_2(x)=\Theta\left(J_2(x)\right)$.
(2) We have $J_1(x)=\Theta\left(J_2(x)\right)$ if and only if $J_2(x)=\Theta\left(J_1(x)\right)$.
(3) If $J_1(x)=\Theta\left(J_2(x)\right)$ and $J_2(x)=\Theta\left(J_3(x)\right)$, then $J_1(x)=\Theta\left(J_3(x)\right)$. The same result holds when $\Theta$ is replaced by $O$ or $\Omega$.
(4) Suppose that $J_1$ and $J_2$ are continuous functions and $J_1(x)=\Theta\left(J_2(x)\right)$. If

$$\liminf_{x\to\infty}\left|J_1(x)\right|>0,$$

then

$$\int_0^x J_1(y)\mathrm{d}y = \Theta\left(\int_0^x J_2(y)\mathrm{d}y\right) \text{ as } x \to \infty.$$

The same result holds for the limit $x \to -\infty$.

*Proof* We only present the proofs of the part 1 and 4. The parts 2 and 3 can be obtained from Chapter 3 of Cormen et al. (2009).
1. Let $\epsilon > 0$ be any positive real number. Note that we have

$$|J_1(x) + J_2(x)| = |J_2(x)| \left| \frac{J_1(x)}{|J_2(x)|} + \frac{J_2(x)}{|J_2(x)|} \right|$$

for all $x \in \mathbb{R}$. Also we have

$$\lim_{x\to\infty} \left| \frac{J_1(x)}{|J_2(x)|} + \frac{J_2(x)}{|J_2(x)|} \right| = 1$$

since $J_1(x) = o\,(J_2(x))$. This implies that there exists $x_1 > 0$ such that

$$|J_1(x) + J_2(x)| \geq (1-\epsilon)\,|J_2(x)|$$

for all $x \geq x_1$. On the other hand, since $J_1(x) = o\,(J_2(x))$, there exists $x_2 > 0$ such that $|J_1(x)| \leq \epsilon\,|J_2(x)|$ for all $x \geq x_2$. This implies that $|J_1(x) + J_2(x)| \leq |J_1(x)| + |J_2(x)| \leq (1+\epsilon)\,|J_2(x)|$ for all $x \geq x_2$. Letting $x' = \max\{x_1, x_2\}$, we have

$$(1-\epsilon)\,|J_2(x)| \leq |J_1(x) + J_2(x)| \leq (1+\epsilon)\,|J_2(x)|$$

for all $x \geq x'$. The asymptotic bound for $x \to -\infty$ can be shown in the same way.
4. By the assumption that $J_1$ is continuous and $\liminf_{x\to\infty} |J_1(x)| > 0$,

$$\exists x_1 > 0 \text{ such that } J_1(x) > 0 \ \ \forall x \geq x_1 \text{ or } J_1(x) < 0 \ \ \forall x \geq x_1. \tag{10}$$

By the assumption that $J_1(x) = \Theta\,(J_2(x))$,

$$\exists a_1, a_2, x_2 > 0 \text{ such that } a_1\,|J_2(x)| \leq |J_1(x)| \leq a_2\,|J_2(x)| \ \text{ for all } x \geq x_2. \tag{11}$$

By this equation and $\liminf_{x\to\infty} |J_1(x)| > 0$, we have $\liminf_{x\to\infty} |J_2(x)| > 0$. This implies that

$$\exists x_3 > 0 \text{ such that } J_2(x) > 0 \ \ \forall x \geq x_3 \text{ or } J_2(x) < 0 \ \ \forall x \geq x_3. \tag{12}$$

Let $x' = \max\{x_1, x_2, x_3\}$. Then we have

$$\left|\int_{x'}^x J_1(y)\mathrm{d}y\right| = \int_{x'}^x |J_1(y)|\,\mathrm{d}y, \quad \left|\int_{x'}^x J_2(y)\mathrm{d}y\right| = \int_{x'}^x |J_2(y)|\,\mathrm{d}y \tag{13}$$

for all $x \geq x'$ by Equations (10) and (12). Now we have

$$a_1 \left| \int_{x'}^{x} J_2(y)\mathrm{d}y \right| \leq \left| \int_{x'}^{x} J_1(y)\mathrm{d}y \right| \leq a_2 \left| \int_{x'}^{x} J_2(y)\mathrm{d}y \right| \tag{14}$$

for all $x \geq x'$ by Equations (11) and (13). Note that we have

$$\begin{aligned} \left| \int_{0}^{x} J_1(y)\mathrm{d}y \right| &\geq \left| \int_{x'}^{x} J_1(y)\mathrm{d}y \right| - \left| \int_{0}^{x'} J_1(y)\mathrm{d}y \right| \\ &\geq a_1 \left| \int_{x'}^{x} J_2(y)\mathrm{d}y \right| - \left| \int_{0}^{x'} J_1(y)\mathrm{d}y \right| \\ &\geq a_1 \left| \int_{0}^{x} J_2(y)\mathrm{d}y \right| - a_1 \left| \int_{0}^{x'} J_2(y)\mathrm{d}y \right| - \left| \int_{0}^{x'} J_1(y)\mathrm{d}y \right| \\ &= \Theta\left( \int_{0}^{x} J_2(y)\mathrm{d}y \right) \end{aligned}$$

for all $x \geq x'$ where the second inequality results from (14) and the last asymptotic equality results from Lemma 1.1.4 since $\liminf_{x\to\infty} |J_2(x)| > 0$ implies $|\int_0^x J_2(y)\mathrm{d}y| \to \infty$ as $x \to \infty$. By Lemma 1.1.3, we have $\int_0^x J_1(y)\mathrm{d}y = \Omega\left(\int_0^x J_2(y)\mathrm{d}y\right)$ as $x \to \infty$. It can be shown in a similar and easier way that $\int_0^x J_1(y)\mathrm{d}y = O\left(\int_0^x J_2(y)\mathrm{d}y\right)$ as $x \to \infty$. These two results imply $\int_0^x J_1(y)\mathrm{d}y = \Theta\left(\int_0^x J_2(y)\mathrm{d}y\right)$ as $x \to \infty$. In the same way, it can be shown that

$$\int_{0}^{x} J_1(y)\mathrm{d}y = \Theta\left( \int_{0}^{x} J_2(y)\mathrm{d}y \right)$$

as $x \to -\infty$. This concludes the proof. ■

Suppose that $F$ is a symmetric distribution. For the $r$-th L-moment $\lambda_r$, we have from Equation (3.51) of Huber and Ronchetti (2009) that

$$\frac{\mathrm{d}}{\mathrm{d}x} \mathrm{IF}\left(x; F, \lambda_r\right) = P^*_{r-1}(F(x)).$$

Note that we have $0 < \lim_{x\to\infty} \left|P^*_{r-1}(F(x))\right| < \infty$ and $0 < \lim_{x\to-\infty} \left|P^*_{r-1}(F(x))\right| < \infty$ by Equation (**??**). This implies $P^*_{r-1}(F(x)) = \Theta(1)$ and further $\int_0^x P^*_{r-1}(F(y))\mathrm{d}y = \Theta(|x|)$ by Lemma 1.1. Then we have $\mathrm{IF}\left(x, F, \lambda_r\right) = \Theta(|x|)$ since $\lim_{x\to\infty} \left|\int_0^x P^*_{r-1}(F(y))\mathrm{d}y\right| = \infty$ holds by $\lim_{x\to\infty} \left|P^*_{r-1}(F(x))\right| > 0$. By Lemma 1.5, we have $\mathrm{IF}\left(x, F, \lambda^*_r\right) = \Theta(|x|)$. By the same steps of derivation, it can be seen that $\mathrm{IF}\left(x, F, \rho^*_r\right) = \Theta(|x|)$.

For the $r$-th HL-moment $\eta_r$, we have from Equation (3.51) of Huber and Ronchetti (2009) that

$$\frac{\mathrm{d}}{\mathrm{d}x} \mathrm{IF}\left(x; T^{0,h}, \eta_r\right) = H_{r-1}\left(\Phi^{-1}(F(x))\right).$$

Let $z(x) = \Phi^{-1}\left(T^{0,h}(x)\right)$. Then we have from Martinez and Iglewicz (1984) that $x = z(x)\exp\left[\left(hz(x)^2\right)/2\right]$. Taking absolute values and logarithm on the both sides yields

$\log|x| = \log|z(x)| + hz(x)^2/2$. Since $z(x) \uparrow \infty$ as $x \to \infty$ and as $x \to -\infty$ and $\log|x| = o\left(x^2\right)$, we have $\log|x| = \Theta\left(z(x)^2\right)$. Then we have $z(x)^2 = \Theta(\log|x|)$ by Lemma 1.1.2, and further $z(x)^2 = \Theta(\log(|x|+1))$ by $\log|x| = \Theta(\log(|x|+1))$ and Lemma 1.1.3. Hence, there exist $x', a_1, a_2 > 0$ such that

$$
\begin{aligned}
&a_1 \log(|x|+1) \le z(x)^2 \le a_2 \log(|x|+1) \text{ for all } |x| \ge x' \\
&\Rightarrow a_1^{1/2}\{\log(|x|+1)\}^{1/2} \le |z(x)| \le a_2^{1/2}\{\log(|x|+1)\}^{1/2} \text{ for all } |x| \ge x'.
\end{aligned}
$$

This implies $z(x) = \Theta\left(\{\log(|x|+1)\}^{1/2}\right)$.

Now let $J(x) = H_{r-1}\left(\Phi^{-1}\left(T^{0,h}(x)\right)\right)$. Then there exist constants $c_{0(r-1)}$, $c_{1(r-1)}$, $\cdots$, $c_{(r-1)(r-1)}$ such that $J(x) = c_{0(r-1)} + c_{1(r-1)}z(x) + \cdots + c_{(r-1)(r-1)}z(x)^{r-1}$. Since $z(x) \uparrow \infty$ implies $z(x)^k = o\left(z(x)^{r-1}\right)$ for all $k = 0, 1, \cdots, r-2$, we have

$$
J(x) = \Theta\left(\{\log(|x|+1)\}^{(r-1)/2}\right) \tag{15}
$$

by Lemma 1.1.1. From Equation (3.50) of Huber and Ronchetti (2009), we have

$$
\mathrm{IF}\left(x; T^{0,h}, \eta_r\right)(x) = l_{T^{0,h}, H_{r-1}\circ T^{0,h}} + \int_0^x J(y)\mathrm{d}y = \Theta\left(\int_0^x J(y)\mathrm{d}y\right) \tag{16}
$$

where the last equality results from Lemma 1.1.1 with $\lim_{x\to\infty}|J(x)| = \lim_{x\to-\infty}|J(x)| = \infty$.

Note that

$$
\begin{aligned}
\int_0^x \{\log(y+1)\}^{(r-1)/2}\mathrm{d}y &= \int_1^{x+1} (\log y)^{(r-1)/2}\mathrm{d}y \\
&= \left[y(\log y)^{(r-1)/2}\right]_1^{x+1} - \frac{r-1}{2}\int_1^{x+1}(\log y)^{(r-3)/2}\mathrm{d}y \\
&= (x+1)\{\log(x+1)\}^{(r-1)/2} - \frac{r-1}{2}\int_1^{x+1}(\log y)^{(r-3)/2}\mathrm{d}y
\end{aligned}
$$

for all $x \ge 0$ where the second equality results from integration by parts. Rearranging the terms yields

$$
(x+1)\{\log(x+1)\}^{(r-1)/2} = \int_1^{x+1}\left\{(\log y)^{(r-1)/2} + \frac{r-1}{2}(\log y)^{(r-3)/2}\right\}\mathrm{d}y.
$$

Since $(\log y)^{(r-3)/2} = o\left((\log y)^{(r-1)/2}\right)$ as $y \to \infty$, we have $(\log y)^{(r-1)/2} + \frac{r-1}{2}(\log y)^{(r-3)/2} = \Theta\left((\log y)^{(r-1)/2}\right)$. Furthermore, since $\lim_{y\to\infty}(\log y)^{(r-1)/2} = \infty$, we have

$$
(x+1)\{\log(x+1)\}^{(r-1)/2} = \Theta\left(\int_1^{x+1}(\log y)^{(r-1)/2}\mathrm{d}y\right) \text{ as } x \to \infty.
$$

By Lemma 1.1.2, we have

$$\int_0^x (\log(y+1))^{(r-1)/2} \mathrm{d}y = \Theta\left((x+1)\{\log(x+1)\}^{(r-1)/2}\right) \text{ as } x \to \infty. \tag{17}$$

By Lemma 1.1.3 with Equations (15), (16) and (17), we have

$$\mathrm{IF}\left(x; T^{0,h}, \eta_r\right) = \Theta\left((|x|+1)\{\log(|x|+1)\}^{(r-1)/2}\right) \text{ as } x \to \infty.$$

By following the same steps of derivation, the same asymptotic bound for the limit $x \to -\infty$ can be obtained. The desired conclusion then follows.

## 1.6. ***Proof of Theorem 5.1***

Serfling (1980) presented asymptotic distributions of functions of random vectors that asymptotically follow multivariate Gaussian distributions.

*Theorem* 1.1 (Theorem 3.3.A of Serfling (1980)) Suppose that $\boldsymbol{X}_n = (X_{n1}, X_{n2}, \cdots, X_{nk})^T$ and $\boldsymbol{X}_n/b_n$ converges in distribution to $\mathcal{N}(\boldsymbol{\mu}, \Sigma)$ where $\boldsymbol{\mu} = (\mu_1, \mu_2, \cdots, \mu_k)$ and $b_n \to 0$ as $n \to \infty$. Let $\boldsymbol{g} : \mathbb{R}^k \to \mathbb{R}^m$ be a vector-valued function such that $\boldsymbol{g}(\boldsymbol{x}) = (g_1(\boldsymbol{x}), g_2(\boldsymbol{x}), \cdots, g_m(\boldsymbol{x}))$ with a nonzero derivative at $\boldsymbol{\mu}$. Then $\boldsymbol{g}\left(\boldsymbol{X}_n\right)/b_n$ converges in distribution to

$$\mathcal{N}\Big(\boldsymbol{g}(\boldsymbol{\mu}), D\Sigma D^T\Big) \tag{18}$$

where $D$ is a matrix whose $(i,j)$-th element is $\mathrm{d}g_i/\mathrm{d}x_j|_{x_j=\mu_j}$. ■

The following lemmas are needed in this subsection.

*Lemma* 1.7 (David and Nagaraja (2003)) Suppose that $E|X|^k < \infty$ for some $k$, then we have

$$\lim_{u\to 1} \left|F^{-1}(u)\right|^k (1-u) = 0, \ \lim_{u\to 0} \left|F^{-1}(u)\right|^k u = 0. \tag{19}$$

This further implies that

$$\lim_{u\to 1} \left|F^{-1}(u)\right|^{sk} (1-u)^s = 0, \quad \lim_{u\to 0} \left|F^{-1}(u)\right|^{sk} u^s = 0 \quad \forall s > 0$$

Moreover, if the CDF $F$ has a MGF, then we have

$$\lim_{u\to 1} \left|F^{-1}(u)\right|^{s} (1-u)^t = 0, \quad \lim_{u\to 0} \left|F^{-1}(u)\right|^{s} u^t = 0 \quad \forall s, t > 0. \tag{20}$$

■

*Lemma* 1.8 (Lemma 3.2.2 of van Zwet (1964)) Suppose that the distribution $F$ satisfies the followings.

(1) Its quantile function $F^{-1}$ is twice differentiable on $(0,1)$ and its second derivative $(F^{-1})''$ is continuous on $(0,1)$.
(2) Its quantile function $F^{-1}$ increases on $(0,1)$.
(3) There exist nonnegative integers $b_1$ and $b_2$ such that $|F^{-1}(t)t^{b_1}(1-t)^{b_2}|$ is bounded on $(0,1)$.

If we have $\lim_{n\to\infty} i_n/n = t$ for some $0 < t < 1$, then $E(X_{i_n:n})$ exists for sufficiently large $n$ and satisfies

$$E(X_{i_n:n}) = F^{-1}\left(\frac{i_n}{n+1}\right) + \frac{1}{2}\frac{1}{n+2}\frac{i_n}{n+1}\left(1-\frac{i_n}{n+1}\right)\left(F^{-1}\right)''\left(\frac{i_n}{n+1}\right) + o\left(\frac{1}{n}\right) \quad (21)$$

as $n \to \infty$. ■

*1.6.1. Asymptotic Gaussianity of the sample HL-moment ratios*

Shorack (1972) showed asymptotic Gaussianity of L-statistics in the form of Equation (4) of the main paper with some conditions on the coefficients $\{c_{ni}|n \geq 1, 1 \leq i \leq n\}$ and the distribution function $F$. We combine Theorem 1 and Example 1 of that paper as the following theorem.

*Theorem* 1.2 (Shorack (1972)) Let $X_1, X_2, \cdots, X_n$ be a random sample generated by the distribution $F$ such that $E|X_1|^k < \infty$ for some positive real number $k$. Let

$$\hat{\theta}_n = \frac{1}{n}\sum_{i=1}^{n} c_{ni}X_{i:n}$$

be an L-statistic of interest. Let $J : (0,1) \to \mathbb{R}$ be a measurable function and $J_n : (0,1) \to \mathbb{R}$ be defined as

$$J_n(t) = \begin{cases} c_{ni} \text{ for } \frac{i-1}{n} < t \leq \frac{i}{n}, \\ c_{n1} \text{ for } t = 0. \end{cases}$$

Suppose that $J$ and $J_n$ satisfy the followings.

(1) There exist $0 < M < \infty, b > 0$ and $\delta > 0$ such that

$$\left|F^{-1}(t)\right| \leq M\{t(1-t)\}^{-1/2+b+\delta},$$
$$|J(t)| \leq M\{t(1-t)\}^{-b},$$
$$|J_n(t)| \leq M\{t(1-t)\}^{-b}$$

for $0 < t < 1$.
(2) Except on a set of $t$'s of $|F^{-1}|$-measure 0, we have both that $J$ is continuous at $t$ and that $J_n$ uniformly converges to $J$ in some neighborhood of $t$ as $n \to \infty$.

(3) We have

$$n^{1/2} \int_0^1 |J_n(u) - J(u)| \left|F^{-1}(u)\right| \, \mathrm{d}u = 0.$$

Then we have

$$\lim_{n\to\infty} n^{1/2} \left(\hat{\theta}_n - \theta\right) \xrightarrow{d} \mathcal{N}\left(0, \sigma^2\right)$$

as $n \to \infty$ where

$$\theta = \int_0^1 J(u)F^{-1}(u)\, \mathrm{d}u, \;\; \sigma^2 = \int_0^1 \int_0^1 (u \wedge v - uv) J(u) J(v)\, \mathrm{d}F^{-1}(u)\, \mathrm{d}F^{-1}(v). \qquad \blacksquare$$

Based on Lemma 1.8, we prove the following lemma.

*Lemma* 1.9 Let $K_r : (0,1) \to \mathbb{R}$ be a function such that $K_r(t) = \left\{\Phi^{-1}(t)\right\}^r$ for $r = 1, 2, \cdots$ and $0 < t < 1$. If we have $\lim_{n\to\infty} i_n/n = t$ for some $0 < t < 1$, then we have

$$E\left(Z^r_{i_n:n}\right) = K_r\left(\frac{i_n}{n+1}\right) + \frac{1}{2}\frac{1}{n+2}\frac{i_n}{n+1}\left(1 - \frac{i_n}{n+1}\right) K_r''\left(\frac{i_n}{n+1}\right) + o\left(\frac{1}{n}\right) \tag{22}$$

for all $r = 1, 2, \cdots$ where the term $o\left(\frac{1}{n}\right)$ does not depend on $i_n$.

*Proof* It can easily be seen that $K_r$ is twice differentiable and its second derivative

$$K_r''(t) = k\frac{(k-1)\left\{\Phi^{-1}(t)\right\}^{k-2} + \left\{\Phi^{-1}(t)\right\}^k}{\left\{\phi\left(\Phi^{-1}(t)\right)\right\}^2}$$

is continuous. Hence $K_r$ satisfies the first condition of Lemma 1.8. It can also be easily seen that the derivative of $K_r$ is positive on $(0,1)$ satisfying the second condition of the lemma.

Let $b > 0$ be any positive integer. It can be seen from Lemma 1.7 that

$$\lim_{t\to 0} t^b \left|K_r(t)\right| = 0 \;\; \lim_{t\to 1} (1-t)^b \left|K_r(t)\right| = 0.$$

This implies that there exist two points $0 < l_r < u_r < 1$ such that

$$\begin{aligned} t^b \left|K_r(t)\right| &\le (1-t)^{-b} \text{ for } 0 < t < l_r \\ (1-t)^b \left|K_r(t)\right| &\le t^{-b} \text{ for } u_r < t < 1. \end{aligned}$$

Since the function $\left|K_r(t)\right| \left\{t(1-t)\right\}^b$ is continuous on $(0,1)$, there exists a constant $0 < \bar{M}_r < \infty$ such that $\left|K_r(t)\right| \left\{t(1-t)\right\}^b \le \bar{M}_r$ for $l_r \le t \le u_r$. Now letting $M_r = \max\{\bar{M}_r, 1\}$ yields

$$|K_r(t)| \le M_r \{t(1-t)\}^{-b}$$

for $0 < t < 1$. This completes the proof. $\blacksquare$

Before we present main results, we present a couple of lemmas below.

*Lemma* 1.10 (Gautschi (1959)) For $x > 0$ and $0 < s < 1$, we have

$$x^{1-s} < \frac{\Gamma(x+1)}{\Gamma(x+s)} < (x+1)^{1-s}. \qquad \blacksquare$$

*Lemma* 1.11 Suppose that $E\left|X_1\right|^{2+\epsilon} < \infty$ for some $\epsilon > 0$. Let

$$\hat{\theta}_{n,r} = \frac{1}{n}\sum_{i=1}^{n} E\left(Z_{i:n}^r\right) X_{i:n}$$

be an L-statistic of interest for $r = 1, 2, \cdots$. Also, let $K_r : (0,1) \to \mathbb{R}$ be a function such that $K_r(t) = \left\{\Phi^{-1}(t)\right\}^r$ for $0 < t < 1$ and $K_{n,r} : (0,1) \to \mathbb{R}$ be defined as

$$K_{n,r}(t) = \begin{cases} E\left(Z_{i:n}^r\right) \text{ for } \frac{i-1}{n} < t \le \frac{i}{n}, \\ E\left(Z_{1:n}^r\right) \text{ for } t = 0. \end{cases}$$

Then $F, K_r$ and $K_{n,r}$ satisfy the three conditions of Theorem 1.2. That is,

(1) There exist $0 < M_r < \infty, b > 0$ and $\delta > 0$ such that

$$\begin{aligned} \left|F^{-1}(t)\right| &\le M_r\{t(1-t)\}^{-1/2+b+\delta}, \\ |K_r(t)| &\le M_r\{t(1-t)\}^{-b}, \\ |K_{n,r}(t)| &\le M_r\{t(1-t)\}^{-b} \end{aligned}$$

for $0 < t < 1$.

(2) Except on a set of $t$'s of $|F^{-1}|$-measure 0, we have both that $J$ is continuous at $t$ and that $J_n$ uniformly converges to $J$ in some neighborhood of $t$ as $n \to \infty$.

(3) We have

$$n^{1/2}\int_0^1 |J_n(u) - J(u)|\left|F^{-1}(u)\right| \mathrm{d}u = 0.$$

*Proof* Let $K_r', K_r'' : (0,1) \to \mathbb{R}$ be the first and second derivatives of the function $K_r$.
<u>Condition 1 of Theorem 1.2</u> Since we have $E\left|X_1\right|^{2+\epsilon} < \infty$, it can be seen from Lemma 1.7 that

$$\lim_{t\to 0} t^{1/(2+\epsilon)}\left|F^{-1}(t)\right| = 0 \ \lim_{t\to 1}(1-t)^{1/(2+\epsilon)}\left|F^{-1}(t)\right| = 0.$$

This implies that there exist two points $0 < l_F < u_F < 1$ such that

$$\begin{aligned} t^{1/(2+\epsilon)}\left|F^{-1}(t)\right| &\le (1-t)^{-1/(2+\epsilon)} \text{ for } 0 < t < l_F \\ (1-t)^{1/(2+\epsilon)}\left|F^{-1}(t)\right| &\le t^{-1/(2+\epsilon)} \text{ for } u_F < t < 1. \end{aligned}$$

Since the function $\left|F^{-1}(t)\right| t^{1/(2+\epsilon)}(1-t)^{1/(2+\epsilon)}$ is continuous on $(0,1)$, there exists a constant $0 < \bar{M}_F < \infty$ such that $\left|F^{-1}(t)\right| t^{1/(2+\epsilon)}(1-t)^{1/(2+\epsilon)} \le \bar{M}_F$ for $l_F \le t \le u_F$. Now letting $\tilde{M}_F = \max\{\bar{M}_F, 1\}$ yields

$$\left|F^{-1}(t)\right| \le \tilde{M}_F t^{-1/(2+\epsilon)}(1-t)^{-1/(2+\epsilon)} \tag{23}$$

for $0 < t < 1$.

Since we have $k = 2+\epsilon$ in Theorem 1.2, there exists $\delta > 0$ such that

$$-\frac{1}{2} + \frac{1}{2+\epsilon} + \delta = -\frac{\epsilon}{2(2+\epsilon)} + \delta < 0.$$

Let $b = \epsilon/\{2(2+\epsilon)\} - \delta > 0$. Since $\epsilon$ can be sufficiently small, we can ensure that $0 < b < 1$. By following the same steps of derivation of the preceding paragraph with Lemma 1.7, it can be seen that there exists $0 < \tilde{M}_r < \infty$ such that

$$|K_r(t)| \le \tilde{M}_r t^{-b}(1-t)^{-b}. \tag{24}$$

Let $0 < t < 1$ be fixed. Note that we have

$$\begin{aligned} E\left(Z^r_{i:n}\right) &= \frac{n!}{(i-1)!(n-i)!}\int_0^1 \left\{\Phi^{-1}(u)\right\}^r u^{i-1}(1-u)^{n-i}\,\mathrm{d}u \\ &= \frac{n!}{(i-1)!(n-i)!}\int_0^1 K_r(u)u^{i-1}(1-u)^{n-i}\,\mathrm{d}u \end{aligned}$$

for all $n \ge 1$ and $1 \le i \le n$. From Equation (24), it can be seen that

$$|K_{n,r}(t)| \le E\left|Z^r_{i:n}\right| = \tilde{M}_r \frac{n!}{(i-1)!(n-i)!}\int_0^1 u^{i-1-b}(1-u)^{n-i-b}\,\mathrm{d}u.$$

where $i$ satisfies $(i-1)/n < t \le i/n$. Note that we have

$$\int_0^1 u^{i-1-b}(1-u)^{n-i-b}\,\mathrm{d}u = \frac{\Gamma(i-b)\Gamma(n-i+1-b)}{\Gamma(n+1-2b)}$$

where $\Gamma$ is the gamma function since the integrand in the left hand side is the density of the distribution $\mathrm{Beta}(i-b, n+1-i-b)$ and $0 < b < 1$. Combining this equation with the preceding equation, we have

$$|K_{n,r}(t)| \le \tilde{M}_r \frac{\Gamma(n+1)}{\Gamma(n+1-2b)}\frac{\Gamma(i-b)}{\Gamma(i)}\frac{\Gamma(n+1-i-b)}{\Gamma(n+1-i)}. \tag{25}$$

Suppose that $\lfloor (n+1)/2 \rfloor \le i \le n-1$. Firstly, substituting $x+1 = i$ and $x+s = i-b$ into Lemma 1.10 yields

$$i^{-b} < \frac{\Gamma(i-b)}{\Gamma(i)} < (i-1)^{-b}$$

since $i \geq 2$ and $0 < 1-b < 1$. Secondly, substituting $x+1 = n+1-i$ and $x+s = n+1-i-b$ into Lemma 1.10 yields

$$(n+1-i)^{-b} < \frac{\Gamma(n+1-i-b)}{\Gamma(n+1-i)} < (n-i)^{-b}$$

since $i \leq n-1$ and $0 < 1-b < 1$. Finally, substituting $x+1 = n+1$ and $x+s = n+1-2b$ into Lemma 1.10 yields

$$n^{2b} < \frac{\Gamma(n+1)}{\Gamma(n+1-2b)} < (n+1)^{2b}$$

since we have $n \geq 1$ and $0 < 1-2b < 1$. By substituting the three preceding equations into Equation (25), we obtain

$$|K_{n,r}(t)| < \tilde{M}_r \left(\frac{n+1}{i-1}\right)^b \left(\frac{n+1}{n-i}\right)^b.$$

Note that

$$\frac{n+1}{i-1}\frac{n+1}{n-i} \leq \frac{2n}{i-1}\frac{2n}{(n-i+1)/2} = 8\frac{n}{i-1}\frac{n}{n-i+1}.$$

Substituting this equation into the preceding equation yields

$$|K_{n,r}(t)| < 8^b \tilde{M}_r \left(\frac{n}{i-1}\right)^b \left(\frac{n}{n-i+1}\right)^b \tag{26}$$

for all $(i-1)/n < t \leq i/n$.

Suppose that $i = n$. Then Equation (25) becomes

$$|K_{n,r}(t)| \leq \tilde{M}_r \frac{\Gamma(n+1)}{\Gamma(n+1-2b)}\frac{\Gamma(n-b)}{\Gamma(n)}\Gamma(1-b). \tag{27}$$

Firstly, substituting $x+1 = n$ and $x+s = n-b$ into Lemma 1.10 yields

$$n^{-b} < \frac{\Gamma(n-b)}{\Gamma(n)} < (n-1)^{-b}$$

since $n \geq 2$ and $0 < 1-b < 1$. Secondly, substituting $x+1 = n+1$ and $x+s = n+1-2b$ into Lemma 1.10 yields

$$n^{2b} < \frac{\Gamma(n+1)}{\Gamma(n+1-2b)} < (n+1)^{2b}$$

since we have $n \geq 1$ and $0 < 1-2b < 1$. Substituting the two preceding inequalities into

Equation (27) yields

$$
\begin{aligned}
|K_{n,r}(t)| &\leq \tilde{M}_r \left(\frac{n+1}{n-1}\right)^b (n+1)^b \Gamma(1-b) \\
&\leq \tilde{M}_r 4^b \Gamma(1-b) \left(\frac{n}{n-1}\right)^b n^b \qquad (28)
\end{aligned}
$$

where the last inequality comes from the fact that $(n+1)/(n-1) \leq 2n/(n-1)$ for all $n \geq 1$.

Combining Equations (26) and (28), we obtain

$$
|K_{n,r}(t)| < \max\left\{\tilde{M}_r 4^b \Gamma(1-b), \tilde{M}_r 8^b\right\} \{t(1-t)\}^{-b}
$$

for $1/2 < t < 1$. By following the same steps of derivation, we obtain the same result for $0 < t \leq 1/2$. Let $M_r = \max\left\{4^b \Gamma(1-b)\tilde{M}_r, 8^b \tilde{M}_r, \tilde{M}_F\right\}$. Then we have

$$
\begin{aligned}
\left|F^{-1}(t)\right| &\leq M_r \{t(1-t)\}^{-1/(2+\epsilon)} = M_r \{t(1-t)\}^{-1/2+b+\delta} \\
|K_r(t)| &\leq M_r \{t(1-t)\}^{-b} \\
|K_{n,r}(t)| &\leq M_r \{t(1-t)\}^{-b}
\end{aligned}
$$

for all $0 < t < 1$.

Condition 2 of Theorem 1.2 The function $K_r$ is continuous on $(0,1)$. Let $s \in (0,1)$ be given. Then there exists $\delta_s > 0$ such that $[s-2\delta_s, s+2\delta_s] \subset (0,1)$. Let $t \in [s-\delta_s, s+\delta_s]$ be fixed. Then we have

$$
\begin{aligned}
|K_r(t) - K_{n,r}(t)| &= \left|K_r(t) - E\left(Z^r_{i_n:n}\right)\right| \\
&\leq \left|K_r(t) - K_r\left(\frac{i_n}{n+1}\right)\right| + \left|K_r\left(\frac{i_n}{n+1}\right) - E\left(Z^r_{i_n:n}\right)\right| \qquad (29)
\end{aligned}
$$

for all $0 < t < 1$ and $1 \leq i_n \leq n$ such that $(i_n - 1)/n < t \leq i_n/n$. Note that $i_n/n \to t$ as $n \to \infty$.

Let $N_1 \geq 1$ be such that $1/N_1 < \delta_s/2$. Then define positive integers $l_n, u_n \geq 1$ for $n \geq N_1$ as

$$
\begin{aligned}
l_n &= \max\left\{1 \leq i \leq n; s - 2\delta_s \leq \frac{i}{n+1} < \frac{i}{n} \leq s - \delta_s\right\}, \\
u_n &= \min\left\{1 \leq i \leq n; s + \delta_s \leq \frac{i}{n+1} < \frac{i}{n} \leq s + 2\delta_s\right\}.
\end{aligned}
$$

Such positive integers exist since $s - 2\delta_s \leq \frac{i}{n} \leq s - \delta_s$ implies either $s - 2\delta_s \leq \frac{i}{n+1} \leq s - \delta_s$ or $s - 2\delta_s \leq \frac{i+1}{n+1} \leq s - \delta_s$ when $n \geq N_1$. Note that $K_r''(t)t(1-t)$ is continuous on the compact set $[s-2\delta_s, s+2\delta_s]$. Hence, there exists

$$
M_s = \sup_{s-2\delta_s \leq t \leq s+2\delta_s} |K_r''(t)|\, t(1-t) < \infty.
$$

Hence, we have by Lemma 1.9 that

$$\begin{aligned}\left|K_r\left(\frac{i_n}{n+1}\right) - E\left(Z^r_{i_n:n}\right)\right| &\leq \frac{1}{2(n+2)}\left|\frac{i_n}{n+1}\left(1-\frac{i_n}{n+1}\right)K_r\left(\frac{i_n}{n+1}\right)\right| + o\left(\frac{1}{n}\right)\\ &\leq \frac{M_s}{2(n+2)} + o\left(\frac{1}{n}\right)\end{aligned}$$

as $n \to \infty$ since we have $s - \delta_s \leq t \leq s + \delta_s$, $(i_n - 1)/n < t \leq i_n/n$ and

$$s - 2\delta_s \leq \frac{l_n}{n} \leq \frac{i_n - 1}{n} < \frac{i_n}{n+1} < \frac{i_n}{n} \leq \frac{u_n}{n} \leq s + 2\delta_s.$$

Hence, there exists $N_2 \geq N_1$ such that

$$\left|K_r\left(\frac{i_n}{n+1}\right) - E\left(Z^r_{i_n:n}\right)\right| < \frac{\epsilon}{2} \tag{30}$$

for all $n \geq N_2$. Note that $N_2$ is independent of $t$.

Since $K_r$ is continuous on the compact set $[s-2\delta_s, s+2\delta_s]$, it is uniformly continuous on that set. This implies that there exists $N_3 \geq 1$ such that $|K_r(t_1) - K_r(t_2)| < \epsilon/2$ holds if $t_1, t_2 \in [s-2\delta_s, s+2\delta_s]$ and $|t_1 - t_2| \leq 1/N_1$. Hence, we have

$$\left|K_r(t) - K_r\left(\frac{i_n}{n+1}\right)\right| \leq \left|K_r\left(\frac{i_n}{n}\right) - K_r\left(\frac{i_n - 1}{n}\right)\right| < \epsilon/2 \tag{31}$$

for all $n \geq N_3$. Note that $N_3$ is independent of $t$.

Substituting this equation and Equations (30) and (31) into Equation (29) yields

$$|K_r(t) - K_{n,r}(t)| < \epsilon$$

for all $s - \delta_s \leq t \leq s + \delta_s$ and $n \geq \max\{N_2, N_3\}$. This implies that $K_{n,r}$ uniformly converges to $K_r$ in some neighborhood of $t$ for all $0 < t < 1$.

<u>Condition 3 of Theorem 1.2</u> Note that

$$\begin{aligned}\frac{1}{x}\phi(x) \geq 1 - \Phi(x)\ \forall x \geq 0 &\Leftrightarrow \frac{1}{x\{1-\Phi(x)\}} \geq \frac{1}{\phi(x)}\ \forall x \geq 0,\\ &\Leftrightarrow \frac{1}{\Phi^{-1}(t)(1-t)} \geq \frac{1}{\phi(\Phi^{-1}(t))}\ \forall 1/2 < t < 1.\end{aligned} \tag{32}$$

We have

$$\begin{aligned}|K_r'(t)| = r\left|\Phi^{-1}(t)\right|^{r-1} \cdot \frac{1}{\phi(\Phi^{-1}(t))} &\leq r\left|\Phi^{-1}(t)\right|^{r-1} \cdot \frac{1}{(1-t)\left|\Phi^{-1}(t)\right|},\\ &= r\left|\Phi^{-1}(t)\right|^{r-2} \cdot \frac{1}{1-t}\end{aligned}$$

for $1/2 \leq t < 1$ which implies that

$$(1-t)^{1+b}\left|K_r'(t)\right| \leq r(1-t)^b\left|\Phi^{-1}(t)\right|^{r-2} \to 0$$

as $t \to 1$ by Lemma 1.7. Similarly, it can be seen that

$$\begin{aligned} & -\frac{1}{x}\phi(x) \geq \Phi(x) \quad \forall x < 0 \\ & \Leftrightarrow -\frac{1}{x\Phi(x)} \geq \frac{1}{\phi(x)} \quad \forall x < 0 \\ & \Leftrightarrow -\frac{1}{t\Phi^{-1}(t)} \geq \frac{1}{\phi(\Phi^{-1}(t))} \quad \forall 0 < t \leq 1/2. \end{aligned} \tag{33}$$

Hence, we have

$$|K_r'(t)| \leq r\left|\Phi^{-1}(t)\right|^{r-1} \cdot \frac{1}{t\left|\Phi^{-1}(t)\right|} = r\left|\Phi^{-1}(t)\right|^{r-2} \cdot \frac{1}{t}$$

which implies that

$$t^{1+b}\left|K_r'(t)\right| \leq rt^b\left|\Phi^{-1}(t)\right|^{r-2} \to 0$$

as $t \to 0$ by Lemma 1.7. This implies that there exist two points $0 < l_r' < u_r' < 1$ such that

$$\begin{aligned} t^{1+b}\left|K_r'(t)\right| &\leq (1-t)^{-1-b} \text{ for } 0 < t < l_r' \\ (1-t)^{1+b}\left|K_r'(t)\right| &\leq t^{-1-b} \text{ for } u_r' < t < 1. \end{aligned}$$

Since the function $|K_r'(t)|\{t(1-t)\}^{1+b}$ is continuous, there exists a constant $0 < \bar{M}_r' < \infty$ such that $|K_r'(t)|\,t^{1+b}(1-t)^{1+b} \leq \bar{M}_r'$ for $l_r' \leq t \leq u_r'$. Now letting $\tilde{M}_r' = \max\{\bar{M}_r', 1\}$ yields

$$|K_r'(t)| \leq \tilde{M}_r'\{t(1-t)\}^{-1-b} \tag{34}$$

for all $0 < t < 1$.

Note that we have

$$K_r''(t) = k\frac{(k-1)\left\{\Phi^{-1}(t)\right\}^{k-2} + \left\{\Phi^{-1}(t)\right\}^k}{\left\{\phi\left(\Phi^{-1}(t)\right)\right\}^2}.$$

By following the same steps of derivation of the preceding paragraph using Equations (32), (33) and Lemma 1.7, it can be seen that there exists $0 < \tilde{M}_r'' < \infty$ such that

$$t(1-t)\left|K_r''(t)\right| \leq \tilde{M}_r''\{t(1-t)\}^{-1-b} \tag{35}$$

for all $0 < t < 1$.

Let $0 < t < 1$ be fixed. Recall from Equation (29) that

$$|K_r(t) - K_{n,r}(t)| \leq \left|K_r(t) - K_r\left(\frac{i_n}{n+1}\right)\right| + \left|K_r\left(\frac{i_n}{n+1}\right) - E\left(Z_{i_n:n}^r\right)\right|.$$

By the mean value theorem, there exists $t^*$ between $i_n/(n+1)$ and $t$ such that

$$\left|K_r\left(\frac{i_n}{n+1}\right)-K_r(t)\right|\leq\left|\frac{i_n}{n+1}-t\right|\left|K_r'\left(t^*\right)\right|$$

Since we have $\left(i_n-1\right)/n\leq i_n/(n+1)\leq i_n/n$, it can be seen that

$$\left|\frac{i_n}{n+1}-t\right|\leq\frac{1}{n} \tag{36}$$

holds. Then there exists $0<\tilde{M}_a<\infty$ such that

$$\begin{aligned}\left|K_r\left(\frac{i_n}{n+1}\right)-K_r(t)\right|&\leq\frac{1}{n}\left|K_r'\left(t^*\right)\right|\\&\leq\frac{1}{n}\tilde{M}_r'\left\{t^*\left(1-t^*\right)\right\}^{-1-b}\\&\leq\frac{1}{n}\tilde{M}_r'\tilde{M}_a\left\{t\left(1-t\right)\right\}^{-1-b}\end{aligned}$$

where the first inequality comes from Equation (36), the second inequality comes from Equation (34) and the last inequality comes from Definition A.3 of Shorack (1972). Using Equation (23), it can be seen that

$$n^{1/2}\left|K_r\left(\frac{i_n}{n+1}\right)-K_r(t)\right|\left|F^{-1}(t)\right|\leq n^{-1/2}\tilde{M}_r'\tilde{M}_a\tilde{M}_F\left\{t\left(1-t\right)\right\}^{-3/2+\delta}. \tag{37}$$

Note that the right hand side does not depend on $i_n$.

Using Lemma 1.9 and Equation (35), we obtain

$$\begin{aligned}&n^{1/2}\left|K_r\left(\frac{i_n}{n+1}\right)-E\left(Z^r_{i_n:n}\right)\right|\left|F^{-1}(t)\right|\\&\leq\frac{n^{1/2}}{2(n+2)}\left\{\frac{i_n}{n+1}\left(1-\frac{i_n}{n+1}\right)\right\}^{-1-b}\left|F^{-1}(t)\right|+n^{1/2}o\left(\frac{1}{n}\right)\left|F^{-1}(t)\right|.\end{aligned}$$

Suppose that $\lfloor(n+1)/2\rfloor\leq i_n\leq n$. Then we have

$$\begin{aligned}\left\{\frac{i_n}{n+1}\left(1-\frac{i_n}{n+1}\right)\right\}^{-1-b}&\leq\left[\frac{2\left(i_n-1\right)}{n}\left\{1-\frac{2\left(i_n-1\right)}{n}\right\}\right]^{-1-b}\\&\leq\left[\frac{2\left(i_n-1\right)}{n}\left\{2-\frac{2\left(i_n-1\right)}{n}\right\}\right]^{-1-b}\\&\leq 4^{-1-b}\left\{\frac{i_n-1}{n}\left(1-\frac{i_n-1}{n}\right)\right\}^{-1-b}.\end{aligned}$$

Hence, we have

$$\left\{\frac{i_n}{n+1}\left(1-\frac{i_n}{n+1}\right)\right\}^{-1-b}\left|F^{-1}(t)\right| \le 4^{-1-b}\left\{\frac{i_n-1}{n}\left(1-\frac{i_n-1}{n}\right)\right\}^{-1-b}\left|F^{-1}(t)\right|$$
$$\le 4^{-1-b}\left|t(1-t)\right|^{-1-b}\left|F^{-1}(t)\right|$$
$$\le 4^{-1-b}\tilde{M}_F\left|t(1-t)\right|^{-1-b}\left|t(1-t)\right|^{-1/2+b+\delta}$$
$$= 4^{-1-b}\tilde{M}_F\left|t(1-t)\right|^{-3/2+\delta}$$

where the second inequality results from $(i_n-1)/n < t$, the third inequality results from Equation (23). We can obtain the same result for $1 \le i_n < \lfloor (n+1)/2 \rfloor$ using $t \le i_n/n$.

Hence, we have

$$n^{1/2}\left|K_r\left(\frac{i}{n+1}\right) - E\left(Z^r_{i:n}\right)\right|\left|F^{-1}(t)\right|$$
$$\le 4^{-1-b}\tilde{M}_F\frac{n^{1/2}}{2(n+2)}\left|t(1-t)\right|^{-3/2+\delta} + n^{1/2}o\left(\frac{1}{n}\right)\left|F^{-1}(t)\right|. \tag{38}$$

Note that the right hand side does not depend on $i_n$. Substituting Equations (37) and (38) into Equation (29) yields

$$n^{1/2}\left|K_r(t) - K_{n,r}(t)\right|\left|F^{-1}(t)\right|$$
$$\le \tilde{M}_F\left\{\tilde{M}'_r\tilde{M}_a n^{-1/2} + 4^{-1-b}\frac{n^{1/2}}{2(n+2)}\right\}\left\{t\left(1-t\right)\right\}^{-3/2+\delta} + n^{1/2}o\left(\frac{1}{n}\right)\left|F^{-1}(t)\right|.$$

By L'Hospital's rule, we have

$$\lim_{n\to\infty} n^{-1/2}\int_{1/n}^{1-1/n}\left\{u(1-u)\right\}^{-3/2-\delta}\,\mathrm{d}u = 0.$$

By the integrability of the random variable $X_1$, we have

$$\int_0^1\left|F^{-1}(u)\right|\,\mathrm{d}u < \infty.$$

Using these two results, we obtain

$$\lim_{n\to\infty} n^{1/2}\int_0^1\left|K_r(t) - K_{n,r}(t)\right|\left|F^{-1}(u)\right|\,\mathrm{d}u = 0. \qquad \blacksquare$$

Based on this lemma, we show asymptotic Gaussianity of a linear combination of the sample HL-moments $\hat{\eta}_r$.

*Lemma* 1.12 Suppose that $E\left|X_1\right|^{2+\epsilon} < \infty$ for some $\epsilon > 0$. Let $c_1, c_2, \cdots, c_r \in \mathbb{R}$ be given and let

$$\bar{\eta}_{n,r} = \sum_{j=1}^r c_j\hat{\eta}_{n,j} = \frac{1}{n}\sum_{j=1}^r c_j\sum_{i=1}^n E\left(H_{j-1}\left(Z_{i:n}\right)\right)X_{i:n}.$$

Then $\bar{\eta}_{n,r}$ satisfies

$$n^{1/2}\left(\bar{\eta}_{n,r}-\sum_{j=1}^{r}c_j\eta_j\right)\xrightarrow{d}\mathcal{N}\left(0,\bar{\sigma}^2\right)$$

as $n\to\infty$ for all $r=1,2,\cdots$ where

$$\bar{\sigma}^2=\int_0^1\int_0^1(u\wedge v-uv)\bar{J}_r(u)\bar{J}_r(v)\,\mathrm{d}F^{-1}(u)\,\mathrm{d}F^{-1}(v),$$
$$\bar{J}_r(t)=\sum_{j=1}^{r}c_jH_{j-1}\left(\Phi^{-1}(t)\right).$$

*Proof* It can be easily seen that there exist constants $a_1,a_2,\cdots,a_r$ such that

$$\bar{J}_r(t)=\sum_{j=1}^{r}a_j\left\{\Phi^{-1}(t)\right\}^{j-1},$$
$$\bar{\eta}_{n,r}=\frac{1}{n}\sum_{j=1}^{r}a_jE\left(Z_{i:n}^{j-1}\right)X_{i:n}.$$

Let $\bar{J}_{n,r}:(0,1)\to\mathbb{R}$ be defined as

$$\bar{J}_{n,r}(t)=\begin{cases}\sum_{j=1}^{r}a_jE\left(Z_{i:n}^{j-1}\right) & \text{for } \frac{i-1}{n}<t\le\frac{i}{n},\\ \sum_{j=1}^{r}a_jE\left(Z_{1:n}^{j-1}\right) & \text{for } t=0.\end{cases}$$

<u>Condition 1 of Theorem 1.2</u> By Result 1 of Lemma 1.11, we have

$$\begin{aligned}|J_r(t)|&\le|a_1|+|a_2|\,M_1\{t(1-t)\}^{-b}+\cdots+|a_{r-1}|\,M_{r-1}\{t(1-t)\}^{-b}\\&=(|a_1|+|a_2|\,M_1+\cdots+|a_{r-1}|\,M_{r-1})\,\{t(1-t)\}^{-b}\\|J_{n,r}(t)|&\le(|a_1|+|a_2|\,M_1+\cdots+|a_{r-1}|\,M_{r-1})\,\{t(1-t)\}^{-b}\end{aligned}$$

Hence, $J_{n,r}$ and $J_r$ satisfy Condition 1 of Theorem 1.2.
<u>Condition 2 of Theorem 1.2</u> By Result 2 of Lemma 1.11, the function $J_r$ is continuous on $(0,1)$ since it is a linear combination of $K_j$ for $0\le j\le r-1$. Also by Result 2 of that lemma, the function $J_{n,r}$ locally uniformly converges to $J_r$ since $J_{n,r}$ is a linear combination of $K_{n,j}$ for $0\le j\le r-1$.
<u>Condition 3 of Theorem 1.2</u> We have

$$\begin{aligned}&n^{1/2}\,|J_{n,r}(t)-J_r(t)|\left|F^{-1}(t)\right|\\&=n^{1/2}\,|a_1+a_2\,\{K_{n,1}(t)-K_1(t)\}+\cdots+a_r\,\{K_{n,r-1}(t)-K_{r-1}(t)\}|\left|F^{-1}(t)\right|\\&=n^{1/2}\,|a_1|\left|F^{-1}(t)\right|+\cdots+n^{1/2}\,|a_r|\,|K_{n,r-1}(t)-K_{r-1}(t)|\left|F^{-1}(t)\right|.\end{aligned}$$

By Result 3 of Lemma 1.11, it can be seen that

$$\lim_{n\to\infty} n^{1/2}\int_0^1 |J_r(t)-J_{n,r}(t)|\left|F^{-1}(u)\right| \,\mathrm{d}u = 0. \qquad \blacksquare$$

We now present the proof of the main result.

*Proof* (Theorem 5.1 of the main paper) By Lemma 1.12 and the Cramér-Wold Theorem, we have

$$n^{1/2}\left(\begin{pmatrix}\hat{\eta}_{n,2}\\ \hat{\eta}_{n,r_1}\\ \hat{\eta}_{n,r_2}\end{pmatrix}-\begin{pmatrix}\eta_2\\ \eta_{r_1}\\ \eta_{r_2}\end{pmatrix}\right)\xrightarrow{d}\mathcal{N}\left(0,\begin{pmatrix}\sigma^H_{22} & \sigma^H_{2r_1} & \sigma^H_{2r_2}\\ \sigma^H_{2r_1} & \sigma^H_{r_1r_1} & \sigma^H_{r_1r_2}\\ \sigma^H_{2r_2} & \sigma^H_{r_2r_1} & \sigma^H_{r_2r_2}\end{pmatrix}\right)$$

as $n\to\infty$ where

$$\begin{aligned}
\sigma^H_{r_ir_j} &= \mathrm{Cov}\left(n^{1/2}\hat{\eta}_{r_i}, n^{1/2}\hat{\eta}_{r_j}\right)\\
&= \frac{1}{2}\left\{\mathrm{Var}(\hat{\eta}_{r_i}+\hat{\eta}_{r_j})-\mathrm{Var}(\hat{\eta}_{r_i})-\mathrm{Var}(\hat{\eta}_{r_j})\right\}\\
&= \frac{1}{2}\left\{\int_0^1\int_0^1 (u\wedge v-uv)\left\{H_{r_i-1}\left(\Phi^{-1}(u)\right)+H_{r_j-1}\left(\Phi^{-1}(u)\right)\right\}\right.\\
&\qquad\qquad \times\left\{H_{r_i-1}\left(\Phi^{-1}(v)\right)+H_{r_j-1}\left(\Phi^{-1}(v)\right)\right\}\,\mathrm{d}F^{-1}(u)\,\mathrm{d}F^{-1}(v)\\
&\qquad -\int_0^1\int_0^1 (u\wedge v-uv)H_{r_i-1}\left(\Phi^{-1}(u)\right)H_{r_i-1}\left(\Phi^{-1}(v)\right)\,\mathrm{d}F^{-1}(u)\,\mathrm{d}F^{-1}(v)\\
&\qquad \left.-\int_0^1\int_0^1 (u\wedge v-uv)H_{r_j-1}\left(\Phi^{-1}(u)\right)H_{r_j-1}\left(\Phi^{-1}(v)\right)\,\mathrm{d}F^{-1}(u)\,\mathrm{d}F^{-1}(v)\right\}\\
&= \int_0^1\int_0^1 (u\wedge v-uv)H_{r_i-1}\left(\Phi^{-1}(u)\right)H_{r_j-1}\left(\Phi^{-1}(v)\right)\,\mathrm{d}F^{-1}(u)\,\mathrm{d}F^{-1}(v)
\end{aligned}$$

where $r_i, r_j\in\{2, r_1, r_2\}$. Now let the function $\boldsymbol{g}=(g_1,g_2)^T$ in Theorem 1.1 be such that $g_1(x_1,x_2,x_3)=x_2/x_1$ and $g_2(x_1,x_2,x_3)=x_3/x_1$. Then we have

$$D=\begin{pmatrix}-\frac{\eta_{r_1}}{\eta_2^2} & -\frac{1}{\eta_2} & 0\\ -\frac{\eta_{r_2}}{\eta_2^2} & 0 & -\frac{1}{\eta_2}\end{pmatrix}$$

Substituting this equation into Equation (18) yields

$$n^{1/2}\left(\begin{pmatrix}\hat{\eta}^*_{n,r_1}\\ \hat{\eta}^*_{n,r_2}\end{pmatrix}-\begin{pmatrix}\eta^*_{r_1}\\ \eta^*_{r_2}\end{pmatrix}\right)\xrightarrow{d}\mathcal{N}\left(\mathbf{0},\Psi^H\right)$$

where $\Psi^H_{i,j}=\left(\sigma^H_{r_ir_j}-\eta^*_{r_i}\sigma^H_{2r_i}-\eta^*_{r_j}\sigma^H_{2r_j}+\eta^*_{r_i}\eta^*_{r_j}\sigma^H_{22}\right)/\eta_2^2$ for $i,j=1,2$. $\blacksquare$

*1.6.2. Asymptotic Gaussianity of the sample RL-skewness and RL-kurtosis*

Since the sample RL-skewness and RL-kurtosis are linear functions of the classical sample L-skewness and L-kurtosis as seen in Equation (23) of the main paper, we have

$$n^{1/2}\left(\begin{pmatrix}\hat{\rho}^*_{n,3}\\ \hat{\rho}^*_{n,4}\end{pmatrix}-\begin{pmatrix}\rho^*_3\\ \rho^*_4\end{pmatrix}\right)\xrightarrow{d}\mathcal{N}\left(\mathbf{0},\Psi^R\right)$$

where

$$\begin{aligned}
\Psi^R &= A\Psi^L A^T\\
A &= \begin{pmatrix}\frac{\delta_{1,2:2}(\Phi)}{\delta_{1,2:3}(\Phi)} & 0\\ 0 & \frac{\delta_{1,2:2}(\Phi)}{5}\left\{\frac{3}{\delta_{2,3:4}(F_0)}+\frac{2}{\delta_{3,4:4}(\Phi)}\right\}\end{pmatrix}\\
\Psi^L_{i,j} &= \left(\sigma^L_{r_ir_j}-\lambda^*_{r_i}\sigma^L_{2r_i}-\lambda^*_{r_j}\sigma^L_{2r_j}+\lambda^*_{r_i}\lambda^*_{r_j}\sigma^L_{22}\right)/\lambda_2^2,\\
\sigma^L_{r_ir_j} &= \int_0^1\int_0^1(u\wedge v-uv)P^*_{r_i-1}(u)P^*_{r_j-1}(v)\,\mathrm{d}F^{-1}(u)\,\mathrm{d}F^{-1}(v)
\end{aligned}$$

for all $i,j\in\{1,2\}$ such that $r_i,r_j\in\{3,4\}$.

## 2. Robustness continued

The following lemma is needed in this section.

*Lemma* 2.1 (Chapter 22, Abramowitz and Stegun (1964)) The Hermite polynomials $\{H_r|r=0,1,2,\cdots\}$ satisfy the recursion formula $(r+1)H_r(x)=\frac{\partial}{\partial x}H_{r+1}(x)$ for $x\in\mathbb{R}$ and $r=0,1,\cdots$. In addition, if $r$ is odd, then $H_r$ is an odd function. If $r$ is even, then $H_r$ is an even function. ■

The following theorem shows the influence functions evaluated at the standard Gaussian distribution.

*Theorem* 2.1 We have

$$\begin{aligned}
\mathrm{IF}\left(x;\Phi,\rho^*_r\right) &= l_{\Phi,R_{r-1}}+\int_0^x R_{r-1}(\Phi(y))\,\mathrm{d}y,\\
\mathrm{IF}\left(x;\Phi,\eta^*_r\right) &= \frac{1}{r}H_r(x)
\end{aligned}$$

for $x\in\mathbb{R}$ and $r=3,4,\cdots$ where

$$l_{F,J}=\int_{-\infty}^0 F(y)J(F(y))\,\mathrm{d}y-\int_0^\infty\{1-F(y)\}J(F(y))\,\mathrm{d}y$$

for $F\in\mathcal{F}$ and a measurable function $J:(0,1)\to\mathbb{R}$.

*Proof* The influence function of the $r$-th RL-moment can directly be obtained from

Equation (3.50) of Huber and Ronchetti (2009). Using Lemma 1.5, it can be shown that $\mathrm{IF}\,(x;\Phi,\rho_r^*) = \mathrm{IF}\,(x;\Phi,\rho_r)$ using the fact that $\rho_2(\Phi) = 1$ and $\rho_r(\Phi) = 0$ for $r = 3, 4, \cdots$.

For the HL-moments, it can be shown that

$$
\begin{aligned}
\mathrm{IF}\,(x;\Phi,\eta_r) &= \int_{-\infty}^{x} \Phi(y) H_{r-1}(y)\,\mathrm{d}y - \int_{x}^{\infty} \{1-\Phi(y)\} H_{r-1}(y)\,\mathrm{d}y \\
&= \left[\frac{1}{r}\Phi(y)H_r(y)\right]_{-\infty}^{x} - \frac{1}{r}\int_{-\infty}^{x} \phi(y)H_r(y)\,\mathrm{d}y \\
&- \left[\frac{1}{r}\{1-\Phi(y)\}H_r(y)\right]_{x}^{\infty} - \frac{1}{r}\int_{x}^{\infty} \phi(y)H_r(y)\,\mathrm{d}y \\
&= \frac{1}{r}H_r(x) - \frac{1}{r}\int_{-\infty}^{\infty} \phi(y)H_r(y)\,\mathrm{d}y \\
&= \frac{1}{r}H_r(x)
\end{aligned}
$$

where the second equality results from Lemma 2.1, the third equality results from Lemma 1.7 and the last equality results from orthogonality of the Hermite polynomials. Using Lemma 1.5, it can be shown that $\mathrm{IF}\,(x;\Phi,\eta_r^*) = \mathrm{IF}\,(x;\Phi,\eta_r) = H_r(x)/r$ since $\eta_2(\Phi) = 1$ and $\eta_r(\Phi) = 0$ for $r = 3, 4, \cdots$. ■

Based on this theorem, it can be seen that

$$
\mathrm{IF}\,(x;\Phi,\eta_3^*) = \frac{1}{3}\mathrm{IF}\,(x;\Phi,\gamma_1)\,,\ \mathrm{SIF}\,(x;\Phi,\eta_4^*) = \frac{1}{4}\mathrm{SIF}\,(x;\Phi,\gamma_2)\,. \tag{39}
$$

The influence function can be understood in some sense as description of local behavior of a functional since it is the directional derivative of a functional with respect to contamination of a distribution by a single point. Equation (39) implies that the HL- and conventional skewness have the same local behavior up to a constant multiple, and the same holds between the HL- and conventional kurtosis.

It can be seen from Theorems 6.1 of the main paper, Lemma 1.1 and Theorem 2.1 of this supplementary material that we have

$$
\begin{aligned}
&|\mathrm{IF}\,(x;\Phi,\gamma_1)| = \Theta\left(|x|^3\right), \quad &&|\mathrm{IF}\,(x;\Phi,\eta_3^*)| = \Theta\left(|x|^3\right), \\
&|\mathrm{SIF}\,(x;\Phi,\gamma_2)| = \Theta\left(|x|^4\right), \quad &&|\mathrm{SIF}\,(x;\Phi,\eta_4^*)| = \Theta\left(|x|^4\right).
\end{aligned}
$$

## 3. TCGA data analysis continued

In this section, we supplement TCGA data analyses done in Section 1 and Subsection 4.1 of the main paper. First, the marginal distribution plots in Figures 1 and 3 of the main paper are reproduced in color in Subsection 3.1, and the marginal distribution plots of genes with the most negative kurtosis estimates are given in Subsection 3.2. Finally, comparison results between different estimators of the HL-moments are given in Subsection 3.3.

### 3.1. *Marginal distribution plots screened by skewness measures in color*

Coloring different subtypes by different shades can help us better understand distributional properties of marginal distributions. Figure 1 shows a colored version of Figure 1 of the main paper. For color specification, see Table 1. Now the colored solid lines are sub-densities corresponding to different subtypes. In the bottom two rows, it can be clearly seen that the Basal-type patients (blue triangles) and Her2-type patients (cyan stars) drive left-skewness of all the genes except GSTT1. The gene GSTT1 has a small cluster of LumA-type patients (red crosses) on the left side of its distribution.

Figure 2 shows a colored version of Figure 3 of the main paper. Again, the Basal-type patients (blue triangles) drive left-skewness of most of the genes in the top two rows. On the contrary, it is hard to see differences in distributions of different subtypes in the bottom two rows. Only the gene DNALI1 has a clear distinction between distributions of the Basal-, Her2-type samples and the samples of the other subtypes.

### 3.2. *Marginal distribution plots screened by kurtosis measures*

In this subsection, we visually compare the performances of different kurtosis estimators in detecting bimodality. As noted in Oja (1981), negatively large values of a kurtosis measure often indicate the bimodality of a distribution. Note that Brown and Hettmansperger (1996) did not show that the negative values of the HL-kurtosis are related to flat shoulders or bimodality. Here we confirm our observation made in Theorem 3.1 based on marginal distribution plots that the HL-kurtosis is actually a measure of kurtosis. Overall, different kurtosis measures considered in this paper do not show much difference in terms of the marginal distributions of the seven genes with the smallest kurtosis estimates. Deeper investigation into relationships between kurtosis estimators in terms of their screening abilities are given in Subsection 4.4 of the main paper.

In Section 6 of the main paper, it was shown that kurtosis measures can be ordered as the conventional, HL-, L- and Ruppert's kurtosis from the least to most robust measures. We first compare the genes with the smallest conventional kurtosis estimates (top two rows) and HL-kurtosis estimates (bottom two rows) in Figure 3. Interestingly, the seven genes with the smallest conventional kurtosis estimates are exactly the same as those with the smallest HL-kurtosis estimates. Overall, all the genes in this figure have multimodality. Some genes such as GSTM1, SLC7A4 and C10orf82 have more than two modes, but generally they are not much peaked at their centers or have heavy shoulders.

Figure 4 shows the seven genes with the smallest L-kurtosis estimates in the top two

| Subtype | LumA | LumB | Her2 | Basal | Normal-like |
|---|---|---|---|---|---|
| Symbol | $+$ | $\times$ | $*$ | $\triangleleft$ | $\triangleright$ |

Table 1.: The symbols and colors corresponding to the 5 subtypes in marginal distribution plots in the Supplementary Material.

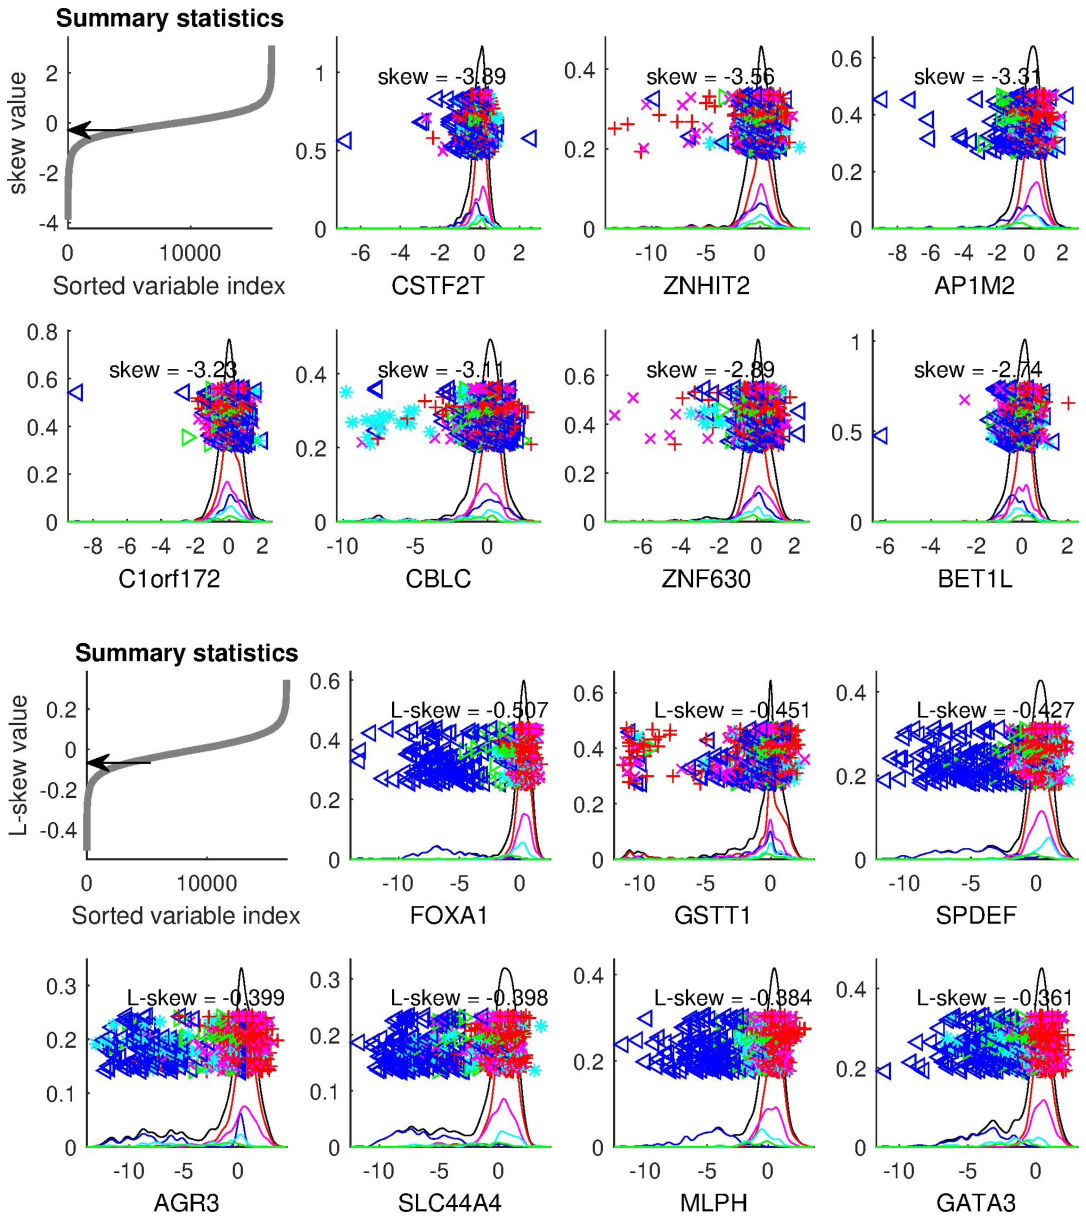


Figure 1.: Color reproduction of Figure 1 of the main paper. It can be clearly seen that distributional skewness in the bottom two rows results from different distributions of different cancer subtypes while the top rows are strongly affected by less biologically interesting outliers.

rows and those with the smallest Ruppert's kurtosis estimates in the bottom two rows. The seven genes screened by the L-kurtosis are a little different from those screened by the conventional and HL-kurtosis estimates given in Figure 3. The three genes NLRP2, PGR and SLC7A4 were not screened by the conventional and HL-kurtosis but are now newly screened by the L-kurtosis. Interestingly, Ruppert's kurtosis screens the seven genes and all of them except the gene RPS28 are the same with the genes of the L-kurtosis.

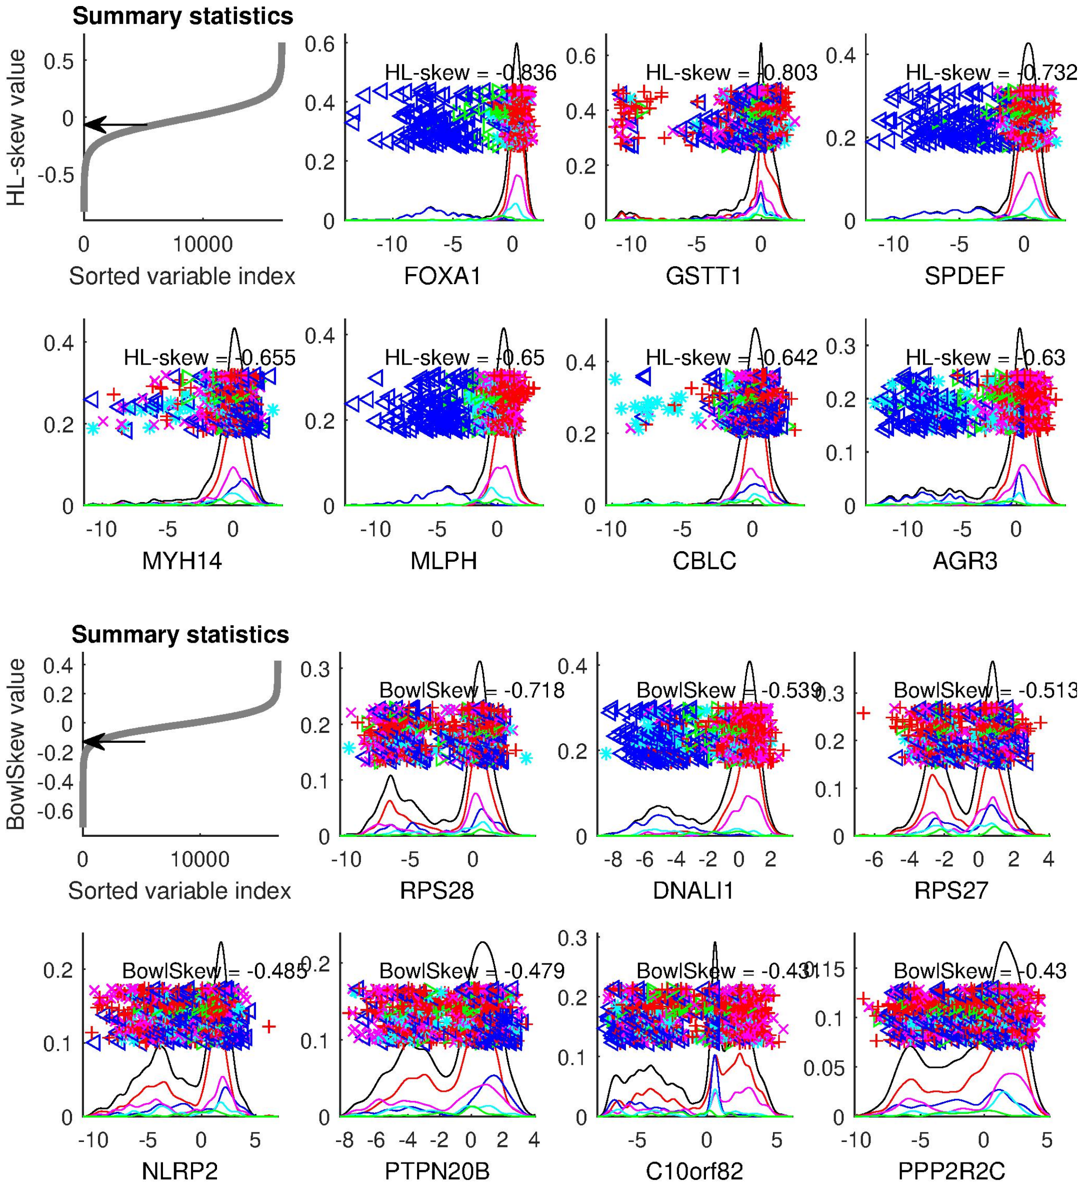


Figure 2.: The marginal distribution plots of seven genes with the smallest sample HL-skewness (top two rows) and Bowley's skewness values (bottom two rows). The seven genes in the top two rows possess distributional skewness to the left side and focus better on subtypes, while those in the bottom two rows sometimes exhibit asymmetric bimodality.

This implies that the conventional and HL-kurtosis share some properties while the L- and Ruppert's kurtosis share some characteristics.

### 3.3. *Comparison between different sample HL-moments by GSEA*

As mentioned in Subsection 3.1 and Section 5 of the main paper, various estimators of the HL-moments can be suggested. In this section, we compare the performances of those

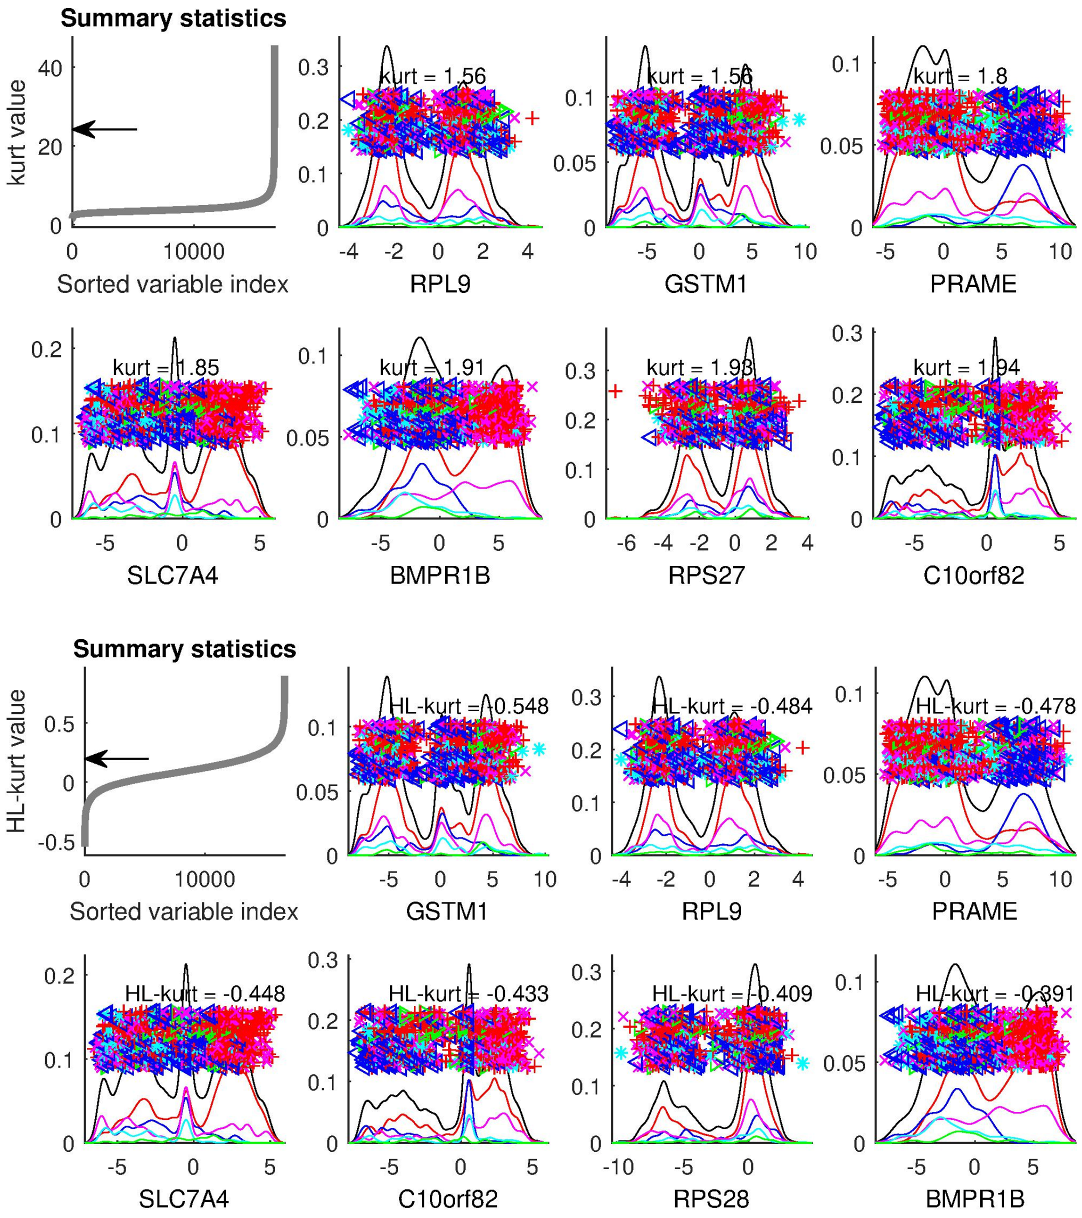


Figure 3.: The marginal distribution plots of seven genes with the smallest conventional kurtosis estimates (top two rows) and HL-kurtosis estimates (bottom two rows). The seven genes in the top two rows are exactly the same with those in the bottom two rows except their relative orders.

estimators by GSEA; see Subsections 4.2, 4.3 and 4.4 of the main paper for detailed

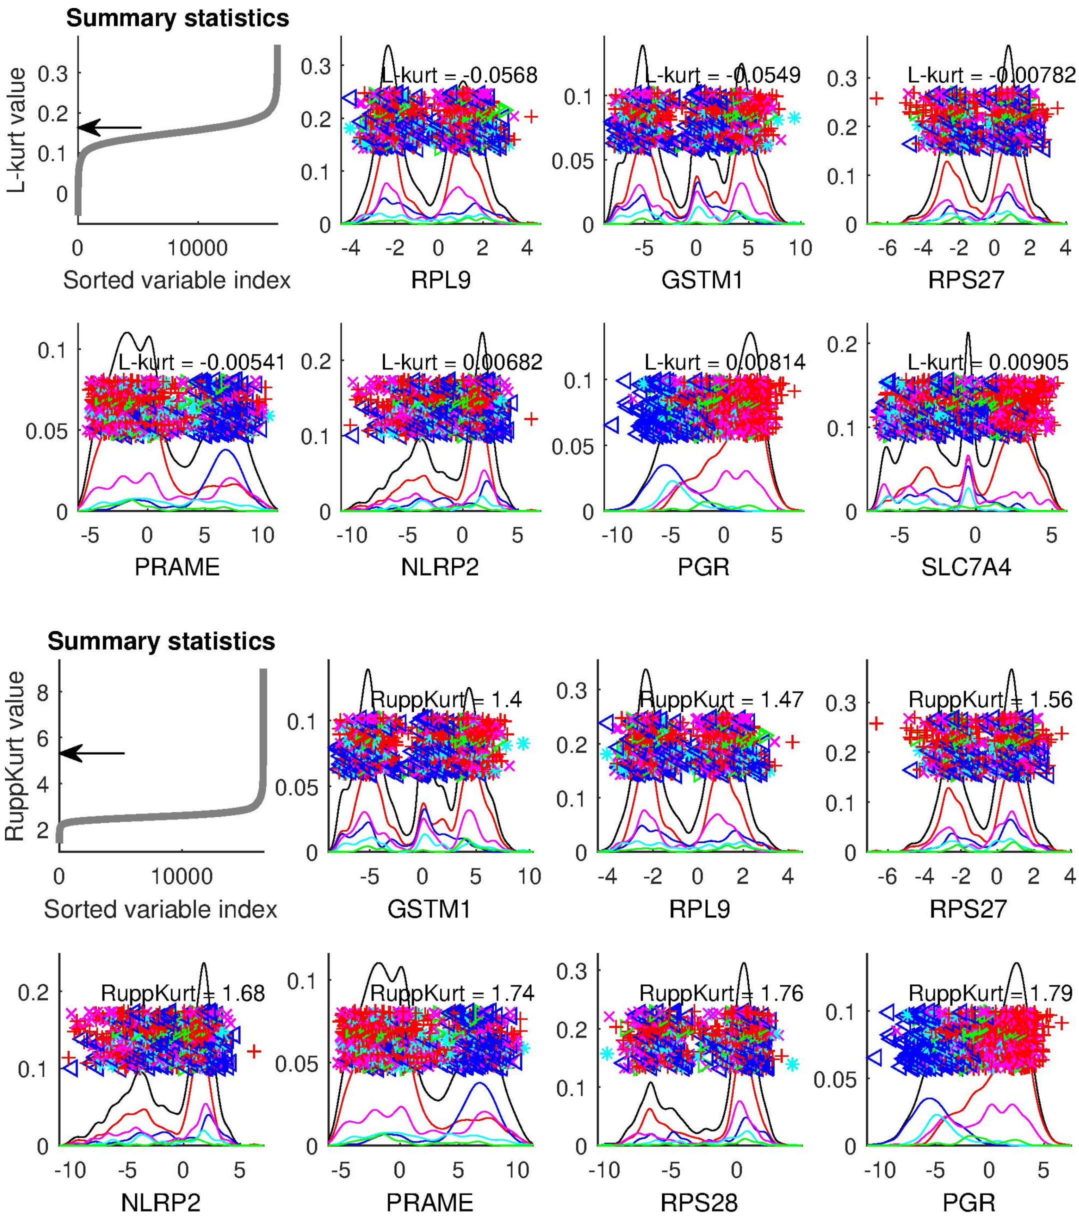


Figure 4.: The marginal distribution plots of seven genes with the smallest L-kurtosis estimates (top two rows) and Ruppert's kurtosis estimates (bottom two rows). The seven genes screened by Ruppert's kurtosis are the same with those screened by the L-kurtosis except the gene RPS28.

explanation. The three estimators of the HL-moments considered herein are

$$\hat{\eta}_r^{(\mathrm{C})} = \frac{1}{n}\sum_{i=1}^{n} H_{r-1}\left(\Phi^{-1}\left(\frac{i}{n+1}\right)\right) X_{i:n},$$

$$\hat{\eta}_r^{(\mathrm{N})} = \frac{1}{n}\sum_{i=1}^{n} E\left(H_{r-1}\left(Z_{i:n}\right)\right) X_{i:n},$$

$$\hat{\eta}_r^{(\mathrm{BH})} = \frac{1}{n}\sum_{i=1}^{n} \left(\int_{(i-1)/n}^{i/n} H_{r-1}\left(\Phi^{-1}(u)\right)\, \mathrm{d}u\right) X_{i:n}.$$

| Estimator (No. of enriched genes) | New (4,992) | Classical (4,856) | Brown-Hettmansperger (4,169) |
|---|---|---|---|
| New (4,992) | | 0.098 | **< 0.001** |
| Classical (4,856) | | | **< 0.001** |

Table 2.: The numbers of gene sets enriched by different HL-kurtosis estimators at the FDR level 0.25 and the significance of their differences based on Fisher's exact test. The new estimator performs the best and BH estimator performs the worst. The superiority of the new estimator over the classical estimator is not significant, but both the new and classical estimators perform significantly better than the Brown-Hettmansberger estimator.

For convenience, we call these estimators the classical estimator $\hat{\eta}_r^{(\mathrm{C})}$, new estimator $\hat{\eta}_r^{(\mathrm{N})}$ and Brown-Hettmansperger (BH) estimator $\hat{\eta}_r^{(\mathrm{BH})}$, respectively. The skewness and kurtosis estimators will be defined as ratios, e.g. $\hat{\eta}_3^{(\mathrm{C})}/\hat{\eta}_2^{(\mathrm{C})}$ and $\hat{\eta}_4^{(\mathrm{C})}/\hat{\eta}_2^{(\mathrm{C})}$. As in Subsections 4.3 and 4.4 of the main paper, we compare the performances of different estimators based on the numbers of interesting gene sets enriched by the ranked lists generated by the estimators. The p-values are then computed by Fisher's exact test.

Comparison between skewness estimators did not show any statistically significant results, so we do not present them here. This implies that choice of coefficients in L-statistics does not affect the performance of skewness estimators much. The comparison results of kurtosis estimators are given in Table 2 with FDR fixed at 0.25. Among the estimators, the new estimator suggested by this paper performs the best, and the BH estimator performs the worst. Since we adopted the new estimator for the HL-moments in comparison between different kurtosis estimators in Subsection 4.4 of the main paper, the number of gene sets enriched by the new estimator in this table is the same with that of Table 5 of the main paper. Note that the inferiority of the BH estimator to the other estimators is statistically significant even after multiple comparison adjustment. Brown and Hettmansperger (1996) claimed that the strength of their estimators is their sensitivity to tail-behavior, but it seems that theirs are too much affected by outliers to be used in our TCGA data analysis. In our analysis, the new estimator seems to best achieve the balance between sensitivity to departure from Gaussianity and robustness to outliers.

Comparison results with the FDR fixed at 0.05 are given in Table 3. The general relationship between different estimators is the same with that of Table 2. The new estimator performs the best and the BW estimator performs the worst. The inferiority of the BW estimators to the other estimators is again statistically significant after multiple comparison adjustment. This result confirms that the new estimator is best for our TCGA analysis.

| Estimator (No. of enriched genes) | New (2,053) | Classical (2,041) | Brown-Hettmansperger (1,679) |
|---|---|---|---|
| New (2,053) | | 0.8535 | **$<$ 0.001** |
| Classical (2,041) | | | **$<$ 0.001** |

Table 3.: The numbers of gene sets enriched by different HL-kurtosis estimators at the FDR level 0.05 and the significance of their differences based on Fisher's exact test. The relationship between the estimators is the same with Table 2; the new estimator performs the best and th BT estimator performs the worst.

## References


Abramowitz, M. and I. A. Stegun (1964). *Handbook of mathematical functions with formulas, graphs, and mathematical tables*, Volume 55 of *National Bureau of Standards Applied Mathematics Series.* For sale by the Superintendent of Documents, U.S. Government Printing Office, Washington, D.C.

Brown, B. M. and T. P. Hettmansperger (1996). Normal scores, normal plots, and tests for normality. *J. Amer. Statist. Assoc. 91*(436), 1668–1675.

Cormen, T. H., C. E. Leiserson, R. L. Rivest, and C. Stein (2009). *Introduction to algorithms* (Third ed.). MIT Press, Cambridge, MA.

David, H. A. and H. N. Nagaraja (2003). *Order statistics* (Third ed.). Wiley Series in Probability and Statistics. Wiley-Interscience John Wiley & Sons, Hoboken, NJ.

Gautschi, W. (1959). Some elementary inequalities relating to the gamma and incomplete gamma function. *J. Math. and Phys. 38*, 77–81.

Hosking, J. R. M. (1989). Some theoretical results concerning l-moments.

Hosking, J. R. M. (1990). $L$-moments: analysis and estimation of distributions using linear combinations of order statistics. *J. Roy. Statist. Soc. Ser. B 52*(1), 105–124.

Huber, P. J. and E. M. Ronchetti (2009). *Robust statistics* (Second ed.). Wiley Series in Probability and Statistics. John Wiley & Sons, Inc., Hoboken, NJ.

Martinez, J. and B. Iglewicz (1984). Some properties of the Tukey $g$ and $h$ family of distributions. *Comm. Statist. A—Theory Methods 13*(3), 353–369.

Oja, H. (1981). On location, scale, skewness and kurtosis of univariate distributions. *Scand. J. Statist. 8*(3), 154–168.

Serfling, R. J. (1980). *Approximation theorems of mathematical statistics.* John Wiley & Sons, Inc., New York. Wiley Series in Probability and Mathematical Statistics.

Shorack, G. R. (1972). Functions of order statistics. *Ann. Math. Statist. 43*, 412–427.

van Zwet, W. R. (1964). *Convex transformations of random variables*, Volume 7 of *Mathematical Centre Tracts.* Mathematisch Centrum, Amsterdam.
